# Supplementary material for: Prevalence of Earth-size Planets Orbiting Sun-like Stars
Source: arXiv:1510.03902 source file (2015-10-13)
Supplement: Supplementary file 1 [file num.tex]

\nc{\rmsteffhuber}{62}
\nc{\rmslogghuber}{0.07}
\nc{\rmsfehuber}{0.10}
\nc{\rmstefftorres}{104}
\nc{\rmsloggtorres}{0.10}
\nc{\rmsfetorres}{0.12}
\nc{\rmsteffspocs}{69}
\nc{\rmsloggspocs}{0.19}
\nc{\rmsfespocs}{0.05}
