# Supplementary material for: Prevalence of Earth-size Planets Orbiting Sun-like Stars
Source: arXiv:1510.03902 source file (2015-10-13)
Supplement: Supplementary file 2 [file table_cks.tex]

KOI-1 &  11446443 & 5782 & 4.36 & -0.06 & < 2.0 &    &     5982 &     4.14 &      P12 \\
    KOI-2 &  10666592 & 6323 & 4.02 &  0.14 &   4.5 &    &     5780 &     4.44 &      Sol \\
    KOI-3 &  10748390 & 4888 & 4.60 &  0.31 & < 2.0 &    &     5780 &     4.44 &      Sol \\
    KOI-6 &   3248033 & 6277 & 4.23 & -0.03 &  11.9 &    &     6557 &     4.31 &      P12 \\
    KOI-7 &  11853905 & 5812 & 4.09 &  0.14 &   2.5 &    &     5961 &     4.34 &      P12 \\
    KOI-8 &   5903312 & 5909 & 4.54 & -0.10 & < 2.0 &    &     6032 &     4.29 &      P12 \\
   KOI-10 &   6922244 & 6242 & 4.14 & -0.11 &  10.4 &    &     6387 &     4.42 &      P12 \\
   KOI-17 &  10874614 & 5732 & 4.29 &  0.36 & < 2.0 &    &     5780 &     4.44 &      Sol \\
   KOI-18 &   8191672 & 6277 & 4.06 & -0.04 &   4.0 &    &     5780 &     4.44 &      Sol \\
   KOI-20 &  11804465 & 5986 & 4.12 &  0.02 &   2.2 &    &     6282 &     4.45 &      P12 \\
   KOI-22 &   9631995 & 5917 & 4.24 &  0.19 & < 2.0 &    &     6076 &     4.49 &      P12 \\
   KOI-41 &   6521045 & 5854 & 4.10 &  0.07 &   2.7 &    &     5932 &     4.51 &      P12 \\
   KOI-42 &   8866102 & 6278 & 4.20 & -0.06 &  13.1 &    &     6228 &     4.22 &      P12 \\
   KOI-46 &  10905239 & 5663 & 4.09 &  0.37 & < 2.0 &    &     5780 &     4.44 &      Sol \\
   KOI-49 &   9527334 & 5831 & 4.33 & -0.09 &   7.5 &    &     5780 &     4.44 &      Sol \\
   KOI-63 &  11554435 & 5659 & 4.68 &  0.22 &   4.8 &    &     5656 &     4.40 &      P12 \\
   KOI-64 &   7051180 & 5362 & 3.86 &  0.03 &   2.1 &    &     5339 &     3.94 &      P12 \\
   KOI-69 &   3544595 & 5579 & 4.26 & -0.17 & < 2.0 &    &     5648 &     4.44 &      P12 \\
   KOI-70 &   6850504 & 5496 & 4.39 &  0.07 & < 2.0 &    &     5540 &     4.58 &      P12 \\
   KOI-72 &  11904151 & 5643 & 4.10 & -0.13 & < 2.0 &    &     5789 &     4.47 &      P12 \\
   KOI-75 &   7199397 & 5880 & 3.86 & -0.13 &   5.0 &    &     6014 &     4.39 &      P12 \\
   KOI-82 &  10187017 & 4911 & 4.64 &  0.09 & < 2.0 &    &     4890 &     3.62 &      P12 \\
   KOI-84 &   2571238 & 5496 & 4.32 & -0.08 & < 2.0 &    &     5623 &     4.57 &      P12 \\
   KOI-85 &   5866724 & 6225 & 4.19 &  0.12 &   8.8 &    &     6266 &     4.07 &      P12 \\
   KOI-87 &  10593626 & 5496 & 4.27 & -0.28 & < 2.0 &    &     5842 &     4.36 &      P12 \\
   KOI-92 &   7941200 & 5961 & 4.41 &  0.05 & < 2.0 &    &     6067 &     4.28 &      P12 \\
   KOI-94 &   6462863 & 6169 & 4.18 &  0.04 &   7.0 &    &     6090 &     4.08 &      KIC \\
   KOI-97 &   5780885 & 6034 & 3.95 &  0.14 &   2.7 &    &     6189 &     4.28 &      P12 \\
   KOI-98 &  10264660 & 6409 & 4.13 & -0.03 &   7.8 &    &     6781 &     3.93 &      P12 \\
   KOI-99 &   8505215 & 5015 & 4.35 & -0.29 & < 2.0 &    &     5162 &     4.53 &      P12 \\
  KOI-102 &   8456679 & 5756 & 4.34 &  0.20 & < 2.0 &    &     6246 &     3.91 &      P12 \\
  KOI-103 &   2444412 & 5568 & 4.41 & -0.03 & < 2.0 &    &     5764 &     4.55 &      P12 \\
  KOI-105 &   8711794 & 5628 & 4.07 & -0.39 & < 2.0 &    &     5810 &     3.96 &      P12 \\
  KOI-107 &  11250587 & 5922 & 4.07 &  0.23 &   3.3 &    &     6055 &     4.47 &      P12 \\
  KOI-108 &   4914423 & 5928 & 4.14 &  0.12 &   3.0 &    &     6141 &     4.36 &      P12 \\
  KOI-110 &   9450647 & 6155 & 4.27 & -0.30 &   6.9 &    &     6539 &     4.36 &      P12 \\
  KOI-111 &   6678383 & 5756 & 4.26 & -0.50 & < 2.0 &    &     6170 &     4.46 &      P12 \\
  KOI-112 &  10984090 & 5883 & 4.37 & -0.06 & < 2.0 &    &     6127 &     4.31 &      P12 \\
  KOI-113 &   2306756 & 5597 & 4.16 &  0.38 & < 2.0 &    &     5495 &     4.40 &      P12 \\
  KOI-115 &   9579641 & 5928 & 4.36 & -0.18 & < 2.0 &    &     6397 &     4.25 &      P12 \\
  KOI-116 &   8395660 & 5920 & 4.40 & -0.11 & < 2.0 &    &     6281 &     3.96 &      P12 \\
  KOI-117 &  10875245 & 5825 & 4.11 &  0.27 &   2.0 &    &     5958 &     4.47 &      P12 \\
  KOI-118 &   3531558 & 5764 & 4.19 &  0.01 & < 2.0 &    &     5907 &     4.50 &      P12 \\
  KOI-119 &   9471974 & 5734 & 4.00 &  0.38 & < 2.0 &    &     5634 &     4.44 &      P12 \\
  KOI-122 &   8349582 & 5716 & 4.20 &  0.27 & < 2.0 &    &     5808 &     4.55 &      P12 \\
  KOI-123 &   5094751 & 5952 & 4.20 & -0.05 & < 2.0 &    &     6153 &     4.28 &      P12 \\
  KOI-124 &  11086270 & 5990 & 4.28 & -0.17 & < 2.0 &    &     6315 &     4.25 &      P12 \\
  KOI-127 &   8359498 & 5533 & 4.34 &  0.30 & < 2.0 &    &     5696 &     4.53 &      P12 \\
  KOI-128 &  11359879 & 5691 & 4.22 &  0.25 & < 2.0 &    &     5839 &     4.18 &      P12 \\
  KOI-134 &   9032900 & 6189 & 4.07 &  0.23 &  10.9 &    &     6368 &     4.39 &      P12 \\
  KOI-135 &   9818381 & 6017 & 4.24 &  0.36 &   4.2 &    &     6145 &     4.47 &      P12 \\
  KOI-137 &   8644288 & 5436 & 4.39 &  0.26 & < 2.0 &    &     5397 &     4.44 &      P12 \\
  KOI-139 &   8559644 & 5946 & 4.33 &  0.19 & < 2.0 &    &     6150 &     4.48 &      P12 \\
  KOI-141 &  12105051 & 5300 & 4.43 &  0.26 & < 2.0 &    &     5403 &     4.60 &      P12 \\
  KOI-142 &   5446285 & 5459 & 4.39 &  0.25 & < 2.0 &    &     5566 &     4.58 &      P12 \\
  KOI-144 &   4180280 & 4913 & 4.53 &  0.23 & < 2.0 &    &     4889 &     3.62 &      P12 \\
  KOI-145 &   9904059 & 4955 & 3.17 &  0.00 &   2.0 &    &     5120 &     3.38 &      P12 \\
  KOI-148 &   5735762 & 5214 & 4.43 &  0.21 & < 2.0 &    &     5189 &     4.52 &      P12 \\
  KOI-149 &   3835670 & 5756 & 4.07 & -0.01 & < 2.0 &    &     5719 &     4.23 &      P12 \\
  KOI-150 &   7626506 & 5501 & 4.11 & -0.51 & < 2.0 &    &     5821 &     4.29 &      P12 \\
  KOI-152 &   8394721 & 6335 & 4.21 & -0.02 &  14.0 &    &     6411 &     4.42 &      P12 \\
  KOI-153 &  12252424 & 4757 & 4.37 &  0.10 & < 2.0 &    &     4743 &     4.63 &      P12 \\
  KOI-155 &   8030148 & 5599 & 3.72 & -0.29 & < 2.0 &    &     5956 &     4.18 &      P12 \\
  KOI-157 &   6541920 & 5805 & 4.39 &  0.03 & < 2.0 &    &     5920 &     4.47 &      P12 \\
  KOI-159 &   8972058 & 6033 & 4.34 & -0.07 &   2.7 &    &     6072 &     4.30 &      P12 \\
  KOI-161 &   5084942 & 4996 & 4.62 &  0.30 & < 2.0 &    &     4903 &     3.66 &      P12 \\
  KOI-162 &   8107380 & 5846 & 4.29 &  0.18 & < 2.0 &    &     5816 &     4.45 &      P12 \\
  KOI-163 &   6851425 & 5082 & 4.39 & -0.42 & < 2.0 &    &     5269 &     4.50 &      P12 \\
  KOI-165 &   9527915 & 5137 & 4.31 & -0.27 & < 2.0 &    &     5199 &     4.64 &      P12 \\
  KOI-166 &   2441495 & 5177 & 4.42 & -0.28 & < 2.0 &    &     5401 &     4.43 &      P12 \\
  KOI-167 &  11666881 & 6265 & 4.17 &  0.02 & < 2.0 &    &     6483 &     4.41 &      P12 \\
  KOI-168 &  11512246 & 5872 & 4.14 & -0.14 & < 2.0 &    &     6143 &     3.97 &      P12 \\
  KOI-171 &   7831264 & 6171 & 4.18 &  0.02 &   7.6 &    &     6499 &     4.40 &      P12 \\
  KOI-172 &   8692861 & 5574 & 3.82 & -0.32 & < 2.0 &    &     5884 &     4.54 &      P12 \\
  KOI-173 &  11402995 & 5733 & 4.30 & -0.02 & < 2.0 &    &     6030 &     4.50 &      P12 \\
  KOI-174 &  10810838 & 4743 & 4.25 & -0.28 & < 2.0 &    &     4876 &     4.61 &      P12 \\
  KOI-176 &   6442377 & 6277 & 4.22 & -0.34 &  10.9 &    &     6561 &     4.39 &      P12 \\
  KOI-177 &   6803202 & 5782 & 4.46 & -0.03 & < 2.0 &    &     5871 &     4.38 &      P12 \\
  KOI-179 &   9663113 & 6098 & 3.95 &  0.17 &   9.0 &    &     6081 &     4.42 &      P12 \\
  KOI-180 &   9573539 & 5673 & 4.59 &  0.02 & < 2.0 &    &     5631 &     4.57 &      P12 \\
  KOI-186 &  12019440 & 5823 & 4.43 &  0.11 & < 2.0 &    &     6087 &     4.50 &      P12 \\
  KOI-191 &   5972334 & 5432 & 4.31 &  0.05 & < 2.0 &    &     5699 &     4.52 &      P12 \\
  KOI-193 &  10799735 & 5496 & 3.26 & -0.36 & < 2.0 &    &     6134 &     4.48 &      P12 \\
  KOI-195 &  11502867 & 5471 & 4.12 & -0.31 & < 2.0 &    &     5865 &     4.50 &      P12 \\
  KOI-197 &   2987027 & 4911 & 4.42 & -0.07 & < 2.0 &    &     5039 &     4.57 &      P12 \\
  KOI-201 &   6849046 & 5539 & 4.32 &  0.30 & < 2.0 &    &     5628 &     4.45 &      P12 \\
  KOI-203 &  10619192 & 5728 & 4.64 &  0.29 &   3.3 &    &     5823 &     4.49 &      P12 \\
  KOI-209 &  10723750 & 6053 & 4.10 & -0.05 &   7.0 &    &     6435 &     4.40 &      P12 \\
  KOI-214 &  11046458 & 5496 & 4.40 &  0.41 & < 2.0 &    &     5476 &     4.44 &      P12 \\
  KOI-232 &   4833421 & 6017 & 4.26 & -0.16 &   3.5 &    &     6095 &     4.49 &      P12 \\
  KOI-237 &   8041216 & 5756 & 4.32 &  0.21 & < 2.0 &    &     5828 &     4.53 &      P12 \\
  KOI-238 &   7219825 & 6135 & 4.23 & -0.17 &   5.2 &    &     6275 &     4.44 &      P12 \\
  KOI-241 &  11288051 & 4896 & 4.06 & -0.56 & < 2.0 &    &     5283 &     4.62 &      P12 \\
  KOI-244 &   4349452 & 6258 & 4.24 & -0.08 &   9.3 &    &     5780 &     4.44 &      Sol \\
  KOI-245 &   8478994 & 5279 & 4.26 & -0.34 & < 2.0 &    &     5780 &     4.44 &      Sol \\
  KOI-246 &  11295426 & 5756 & 4.17 &  0.10 & < 2.0 &    &     5795 &     4.42 &      P12 \\
  KOI-257 &   5514383 & 6181 & 4.28 &  0.06 &   7.3 &    &     6257 &     4.09 &      P12 \\
  KOI-260 &   8292840 & 6211 & 4.24 & -0.26 &   8.6 &    &     5780 &     4.44 &      Sol \\
  KOI-261 &   5383248 & 5784 & 4.61 &  0.08 & < 2.0 &    &     5777 &     3.96 &      P12 \\
  KOI-262 &  11807274 & 6184 & 4.18 & -0.14 &  10.0 &    &     6416 &     4.24 &      P12 \\
  KOI-263 &  10514430 & 5781 & 4.08 & -0.18 & < 2.0 &    &     5860 &     4.34 &      P12 \\
  KOI-265 &  12024120 & 6022 & 4.22 &  0.11 &   2.2 &    &     6274 &     4.37 &      P12 \\
  KOI-266 &   7375348 & 6184 & 4.29 & -0.10 &   5.4 &    &     5780 &     4.44 &      Sol \\
  KOI-268 &   3425851 & 6375 & 4.17 & -0.07 &   8.5 &    &     5780 &     4.44 &      Sol \\
  KOI-269 &   7670943 & 6277 & 4.22 & -0.16 &  11.6 &    &     6521 &     4.12 &      P12 \\
  KOI-270 &   6528464 & 5671 & 4.01 & -0.19 &   3.0 &    &     5780 &     4.44 &      Sol \\
  KOI-271 &   9451706 & 6157 & 4.20 &  0.24 &   6.1 &    &     6298 &     4.45 &      P12 \\
  KOI-273 &   3102384 & 5726 & 4.36 &  0.29 & < 2.0 &    &     5656 &     4.57 &      P12 \\
  KOI-274 &   8077137 & 6049 & 4.06 & -0.09 &   6.1 &    &     6247 &     4.36 &      P12 \\
  KOI-275 &  10586004 & 5813 & 4.05 &  0.22 & < 2.0 &    &     5780 &     4.44 &      Sol \\
  KOI-276 &  11133306 & 5994 & 4.28 & -0.06 & < 2.0 &    &     6194 &     4.36 &      P12 \\
  KOI-277 &  11401755 & 6001 & 4.15 & -0.24 &   4.4 &    &     5780 &     4.44 &      Sol \\
  KOI-279 &  12314973 & 6266 & 4.15 &  0.11 &  13.0 &    &     6419 &     4.28 &      P12 \\
  KOI-280 &   4141376 & 6017 & 4.40 & -0.37 & < 2.0 &    &     6315 &     4.21 &      P12 \\
  KOI-281 &   4143755 & 5606 & 3.69 & -0.47 & < 2.0 &    &     6091 &     3.89 &      P12 \\
  KOI-282 &   5088536 & 5776 & 4.18 & -0.30 & < 2.0 &    &     5780 &     4.44 &      Sol \\
  KOI-283 &   5695396 & 5791 & 4.50 &  0.17 & < 2.0 &    &     5875 &     3.99 &      P12 \\
  KOI-284 &   6021275 & 5943 & 4.39 & -0.29 & < 2.0 &    &     6177 &     4.14 &      P12 \\
  KOI-285 &   6196457 & 6011 & 4.10 &  0.18 &   3.0 &    &     5780 &     4.44 &      Sol \\
  KOI-288 &   9592705 & 6193 & 4.00 &  0.18 &   7.5 &    &     5780 &     4.44 &      Sol \\
  KOI-289 &  10386922 & 5866 & 4.05 & -0.42 & < 2.0 &    &     5780 &     4.44 &      Sol \\
  KOI-291 &  10933561 & 5724 & 4.20 &  0.26 &   3.1 &    &     5685 &     4.57 &      P12 \\
  KOI-292 &  11075737 & 5756 & 4.43 & -0.23 & < 2.0 &    &     6027 &     4.25 &      P12 \\
  KOI-294 &  11259686 & 6025 & 4.29 & -0.03 &   4.4 &    &     6125 &     4.45 &      P12 \\
  KOI-295 &  11547513 & 5962 & 4.48 & -0.25 & < 2.0 &    &     5780 &     4.44 &      Sol \\
  KOI-296 &  11802615 & 5756 & 4.33 & -0.19 & < 2.0 &    &     6089 &     4.39 &      P12 \\
  KOI-297 &  11905011 & 6137 & 4.19 &  0.04 &   6.9 &    &     6281 &     4.28 &      P12 \\
  KOI-299 &   2692377 & 5544 & 4.52 &  0.17 & < 2.0 &    &     5711 &     3.97 &      P12 \\
  KOI-301 &   3642289 & 6029 & 4.10 & -0.13 &   5.1 &    &     6336 &     4.33 &      P12 \\
  KOI-303 &   5966322 & 5587 & 4.14 & -0.21 & < 2.0 &    &     5734 &     4.51 &      P12 \\
  KOI-304 &   6029239 & 5756 & 4.51 & -0.25 & < 2.0 &    &     6150 &     3.98 &      P12 \\
  KOI-305 &   6063220 & 4839 & 4.55 &  0.21 & < 2.0 &    &     4747 &     4.63 &      P12 \\
  KOI-306 &   6071903 & 5344 & 4.67 &  0.13 & < 2.0 &    &     5275 &     3.96 &      P12 \\
  KOI-307 &   6289257 & 6017 & 4.42 & -0.17 &   5.1 &    &     6315 &     4.40 &      P12 \\
  KOI-308 &   6291837 & 6226 & 4.29 & -0.04 &  10.0 &    &     6357 &     4.13 &      P12 \\
  KOI-312 &   7050989 & 6178 & 4.15 & -0.01 &   9.5 &    &     5780 &     4.44 &      Sol \\
  KOI-313 &   7419318 & 5242 & 4.43 &  0.01 & < 2.0 &    &     5340 &     4.46 &      P12 \\
  KOI-315 &   7700622 & 4814 & 4.48 & -0.25 & < 2.0 &    &     4875 &     4.61 &      P12 \\
  KOI-316 &   8008067 & 5542 & 4.16 &  0.30 & < 2.0 &    &     5703 &     4.33 &      P12 \\
  KOI-317 &   8121310 & 6508 & 4.18 &  0.01 &  16.0 &    &     6659 &     4.06 &      P12 \\
  KOI-318 &   8156120 & 6298 & 4.07 &  0.21 &  13.5 &    &     6580 &     4.26 &      P12 \\
  KOI-319 &   8684730 & 5945 & 3.99 &  0.11 &   4.8 &    &     5780 &     4.44 &      Sol \\
  KOI-321 &   8753657 & 5664 & 4.32 &  0.26 & < 2.0 &    &     5614 &     4.57 &      P12 \\
  KOI-323 &   9139084 & 5484 & 4.67 &  0.01 &   4.1 &    &     5565 &     4.34 &      P12 \\
  KOI-327 &   9881662 & 6054 & 4.28 & -0.08 &   4.0 &    &     6355 &     4.42 &      P12 \\
  KOI-328 &   9895004 & 5894 & 4.57 & -0.06 & < 2.0 &    &     5821 &     4.45 &      P12 \\
  KOI-330 &  11361646 & 5853 & 4.07 & -0.04 & < 2.0 &    &     6027 &     4.26 &      P12 \\
  KOI-331 &  10285631 & 5496 & 3.83 &  0.05 & < 2.0 &    &     5556 &     4.58 &      P12 \\
  KOI-332 &  10290666 & 5774 & 4.18 &  0.33 &   2.0 &    &     5757 &     4.55 &      P12 \\
  KOI-333 &  10337258 & 6183 & 4.27 &  0.03 &   8.0 &    &     6540 &     4.39 &      P12 \\
  KOI-337 &  10545066 & 5765 & 4.34 &  0.04 & < 2.0 &    &     6010 &     4.51 &      P12 \\
  KOI-338 &  10552611 & 5008 & 4.56 &  0.32 & < 2.0 &    &     4973 &     3.78 &      P12 \\
  KOI-339 &  10587105 & 5962 & 4.43 & -0.27 &   4.7 &    &     6274 &     4.45 &      P12 \\
  KOI-340 &  10616571 & 5718 & 4.19 &  0.33 &   6.7 &    &     5717 &     3.86 &      P12 \\
  KOI-341 &  10878263 & 5553 & 4.55 &  0.13 & < 2.0 &    &     5585 &     4.32 &      P12 \\
  KOI-343 &  10982872 & 5756 & 4.32 & -0.00 & < 2.0 &    &     5946 &     4.44 &      P12 \\
  KOI-344 &  11015108 & 5534 & 4.20 & -0.30 & < 2.0 &    &     5981 &     4.34 &      P12 \\
  KOI-345 &  11074541 & 4911 & 4.50 &  0.03 & < 2.0 &    &     4939 &     3.74 &      P12 \\
  KOI-346 &  11100383 & 5121 & 4.66 &  0.05 & < 2.0 &    &     5109 &     4.55 &      P12 \\
  KOI-348 &  11194032 & 4782 & 4.52 &  0.07 & < 2.0 &    &     4742 &     4.63 &      P12 \\
  KOI-349 &  11394027 & 5756 & 4.33 &  0.30 &   3.3 &    &     5813 &     4.37 &      P12 \\
  KOI-350 &  11395587 & 5817 & 4.51 &  0.02 & < 2.0 &    &     6017 &     4.38 &      P12 \\
  KOI-351 &  11442793 & 6017 & 4.27 &  0.06 &   3.6 &    &     6317 &     4.43 &      P12 \\
  KOI-352 &  11521793 & 5831 & 4.20 & -0.07 & < 2.0 &    &     6001 &     4.39 &      P12 \\
  KOI-355 &  11621223 & 6104 & 4.21 &  0.14 &   4.1 &    &     6282 &     4.43 &      P12 \\
  KOI-356 &  11624249 & 5441 & 4.34 & -0.03 & < 2.0 &    &     5369 &     3.99 &      P12 \\
  KOI-360 &  12107021 & 6017 & 4.32 & -0.18 & < 2.0 &    &     5780 &     4.44 &      Sol \\
  KOI-361 &  12404954 & 5662 & 4.33 &  0.10 & < 2.0 &    &     5922 &     4.53 &      P12 \\
  KOI-364 &   7296438 & 5821 & 4.14 &  0.25 & < 2.0 &    &     5750 &     4.45 &      P12 \\
  KOI-365 &  11623629 & 5483 & 4.34 & -0.14 & < 2.0 &    &     5611 &     4.57 &      P12 \\
  KOI-367 &   4815520 & 5756 & 4.47 &  0.15 & < 2.0 &    &     5864 &     4.32 &      P12 \\
  KOI-369 &   7175184 & 6132 & 4.26 & -0.25 &   6.5 &    &     6372 &     4.41 &      P12 \\
  KOI-370 &   8494142 & 6036 & 4.01 & -0.02 &   6.4 &    &     6520 &     3.83 &      P12 \\
  KOI-371 &   5652983 & 5176 & 3.56 &  0.07 & < 2.0 &    &     5223 &     3.60 &      P12 \\
  KOI-372 &   6471021 & 5831 & 4.64 & -0.05 &   3.2 &    &     5921 &     4.50 &      P12 \\
  KOI-373 &   7364176 & 5757 & 4.43 & -0.42 & < 2.0 &    &     6121 &     4.26 &      P12 \\
  KOI-374 &   8686097 & 5756 & 4.18 & -0.31 & < 2.0 &    &     6095 &     4.29 &      P12 \\
  KOI-375 &  12356617 & 5756 & 4.06 &  0.15 & < 2.0 &    &     5966 &     4.43 &      P12 \\
  KOI-377 &   3323887 & 5838 & 4.58 &  0.07 & < 2.0 &    &     5866 &     4.54 &      P12 \\
  KOI-379 &   2446113 & 6112 & 3.97 &  0.12 &   7.3 &    &     6554 &     4.12 &      P12 \\
  KOI-384 &   3353050 & 6020 & 3.85 & -0.09 &   5.5 &    &     6075 &     4.29 &      P12 \\
  KOI-385 &   3446746 & 5455 & 4.34 &  0.08 & < 2.0 &    &     5642 &     4.43 &      P12 \\
  KOI-386 &   3656121 & 5989 & 4.39 &  0.00 &   3.3 &    &     6212 &     4.38 &      P12 \\
  KOI-387 &   3733628 & 4783 & 4.61 & -0.05 & < 2.0 &    &     5780 &     4.44 &      Sol \\
  KOI-388 &   3831053 & 5772 & 4.00 &  0.06 &   2.4 &    &     5780 &     4.44 &      Sol \\
  KOI-392 &   3942670 & 5983 & 4.15 &  0.06 &   3.8 &    &     5892 &     4.27 &      P12 \\
  KOI-393 &   3964109 & 6164 & 4.17 & -0.32 &   7.7 &    &     6262 &     4.46 &      P12 \\
  KOI-399 &   7289157 & 6108 & 4.37 & -0.06 &   6.2 &    &     6281 &     4.20 &      P12 \\
  KOI-401 &   3217264 & 5453 & 4.43 &  0.33 & < 2.0 &    &     5376 &     4.00 &      P12 \\
  KOI-403 &   4247092 & 6248 & 4.14 & -0.01 &  10.0 &    &     5785 &     4.44 &      P12 \\
  KOI-408 &   5351250 & 5548 & 4.45 &  0.02 & < 2.0 &    &     5855 &     4.48 &      P12 \\
  KOI-409 &   5444548 & 5859 & 4.39 &  0.13 & < 2.0 &    &     5883 &     4.53 &      P12 \\
  KOI-415 &   6289650 & 5699 & 3.99 & -0.28 & < 2.0 &    &     6082 &     4.36 &      P12 \\
  KOI-416 &   6508221 & 5058 & 4.43 & -0.23 & < 2.0 &    &     5249 &     4.63 &      P12 \\
  KOI-427 &  10189546 & 5357 & 4.60 &  0.07 & < 2.0 &    &     5462 &     4.50 &      P12 \\
  KOI-431 &  10843590 & 5148 & 4.39 & -0.36 & < 2.0 &    &     5417 &     4.43 &      P12 \\
  KOI-433 &  10937029 & 5167 & 4.33 &  0.09 & < 2.0 &    &     5269 &     4.49 &      P12 \\
  KOI-435 &  11709124 & 5624 & 4.12 & -0.09 & < 2.0 &    &     5991 &     4.51 &      P12 \\
  KOI-439 &  12470954 & 5446 & 4.35 &  0.31 & < 2.0 &    &     5355 &     4.61 &      P12 \\
  KOI-440 &   2438264 & 5085 & 4.56 &  0.13 & < 2.0 &    &     5031 &     4.57 &      P12 \\
  KOI-442 &   3745690 & 5809 & 4.33 & -0.08 & < 2.0 &    &     5969 &     4.52 &      P12 \\
  KOI-444 &   3847138 & 5679 & 4.35 & -0.11 & < 2.0 &    &     5935 &     4.51 &      P12 \\
  KOI-456 &   7269974 & 5589 & 4.26 &  0.14 & < 2.0 &    &     5889 &     4.51 &      P12 \\
  KOI-457 &   7440748 & 5125 & 4.62 &  0.21 & < 2.0 &    &     5058 &     4.65 &      P12 \\
  KOI-459 &   7977197 & 5862 & 4.31 &  0.03 &   2.1 &    &     5833 &     4.44 &      P12 \\
  KOI-465 &   8891318 & 6029 & 4.18 & -0.06 &   3.5 &    &     6235 &     4.46 &      P12 \\
  KOI-466 &   9008220 & 5950 & 4.13 & -0.05 &   5.9 &    &     6116 &     4.49 &      P12 \\
  KOI-474 &  10460984 & 6005 & 4.45 & -0.03 & < 2.0 &    &     6360 &     4.42 &      P12 \\
  KOI-475 &  10577994 & 5116 & 4.53 & -0.38 & < 2.0 &    &     5236 &     4.54 &      P12 \\
  KOI-479 &  11015323 & 5552 & 4.28 & -0.11 & < 2.0 &    &     5823 &     4.53 &      P12 \\
  KOI-486 &  12404305 & 5670 & 4.14 & -0.38 & < 2.0 &    &     5908 &     4.53 &      P12 \\
  KOI-490 &   3239945 & 4849 & 4.47 & -0.02 & < 2.0 &    &     4911 &     4.60 &      P12 \\
  KOI-505 &   5689351 & 5041 & 4.62 &  0.11 & < 2.0 &    &     5074 &     3.86 &      P12 \\
  KOI-508 &   6266741 & 5538 & 4.34 &  0.32 & < 2.0 &    &     5614 &     4.26 &      P12 \\
  KOI-509 &   6381846 & 5564 & 4.54 &  0.09 & < 2.0 &    &     5631 &     4.57 &      P12 \\
  KOI-510 &   6422155 & 5573 & 4.31 &  0.35 & < 2.0 &    &     5543 &     4.39 &      P12 \\
  KOI-517 &   8015907 & 5547 & 4.58 &  0.20 & < 2.0 &    &     5669 &     4.32 &      P12 \\
  KOI-518 &   8017703 & 4756 & 4.24 & -0.63 & < 2.0 &    &     5037 &     4.60 &      P12 \\
  KOI-523 &   8806123 & 5644 & 3.83 & -0.23 & < 2.0 &    &     6199 &     4.42 &      P12 \\
  KOI-528 &   9941859 & 5365 & 4.31 & -0.10 & < 2.0 &    &     5675 &     4.34 &      P12 \\
  KOI-534 &  10554999 & 5291 & 4.55 &  0.06 & < 2.0 &    &     5283 &     4.63 &      P12 \\
  KOI-543 &  11823054 & 5119 & 4.38 & -0.11 & < 2.0 &    &     5327 &     4.62 &      P12 \\
  KOI-548 &  12600735 & 6015 & 4.23 & -0.11 & < 2.0 &    &     6359 &     4.43 &      P12 \\
  KOI-550 &   4165473 & 5702 & 4.42 &  0.13 & < 2.0 &    &     5869 &     4.54 &      P12 \\
  KOI-555 &   5709725 & 5257 & 4.34 &  0.04 & < 2.0 &    &     5408 &     4.60 &      P12 \\
  KOI-561 &   6665695 & 5015 & 4.30 & -0.22 & < 2.0 &    &     5234 &     4.59 &      P12 \\
  KOI-564 &   6786037 & 5845 & 4.04 &  0.27 &   4.1 &    &     5951 &     4.52 &      P12 \\
  KOI-568 &   7595157 & 5297 & 4.29 & -0.01 & < 2.0 &    &     5386 &     4.61 &      P12 \\
  KOI-569 &   8008206 & 5055 & 4.57 & -0.23 & < 2.0 &    &     5174 &     4.55 &      P12 \\
  KOI-572 &   8193178 & 6005 & 4.11 & -0.11 &   4.0 &    &     5977 &     4.32 &      P12 \\
  KOI-573 &   8344004 & 5667 & 4.28 &  0.08 & < 2.0 &    &     6010 &     4.34 &      P12 \\
  KOI-574 &   8355239 & 5075 & 4.45 & -0.10 & < 2.0 &    &     5217 &     4.63 &      P12 \\
  KOI-577 &   8558011 & 5074 & 4.44 &  0.05 & < 2.0 &    &     5043 &     4.31 &      KIC \\
  KOI-579 &   8616637 & 5145 & 4.60 &  0.01 & < 2.0 &    &     5194 &     4.61 &      P12 \\
  KOI-584 &   9146018 & 5496 & 4.34 &  0.26 & < 2.0 &    &     5525 &     4.59 &      P12 \\
  KOI-590 &   9782691 & 5975 & 4.38 & -0.08 &   3.5 &    &     6308 &     4.44 &      P12 \\
  KOI-598 &  10656823 & 5288 & 4.61 &  0.01 & < 2.0 &    &     5292 &     4.62 &      P12 \\
  KOI-600 &  10718726 & 5762 & 4.28 & -0.10 & < 2.0 &    &     6085 &     4.45 &      P12 \\
  KOI-611 &   6309763 & 6351 & 4.26 &  0.05 &  12.2 &    &     6365 &     4.43 &      P12 \\
  KOI-612 &   6587002 & 5157 & 4.52 & -0.03 & < 2.0 &    &     5259 &     4.50 &      P12 \\
  KOI-620 &  11773022 & 5660 & 4.59 & -0.03 &   5.4 &    &     6023 &     4.51 &      P12 \\
  KOI-623 &  12068975 & 5866 & 4.19 & -0.56 & < 2.0 &    &     6475 &     4.08 &      P12 \\
  KOI-624 &   3541946 & 5698 & 4.62 &  0.08 & < 2.0 &    &     5725 &     4.56 &      P12 \\
  KOI-626 &   4478168 & 6017 & 4.24 & -0.31 &   3.3 &    &     6387 &     4.39 &      P12 \\
  KOI-627 &   4563268 & 6017 & 4.15 &  0.13 &   5.0 &    &     6067 &     4.22 &      P12 \\
  KOI-628 &   4644604 & 5674 & 4.10 & -0.44 & < 2.0 &    &     6022 &     4.24 &      P12 \\
  KOI-629 &   4656049 & 6017 & 4.22 & -0.39 & < 2.0 &    &     6459 &     4.18 &      P12 \\
  KOI-632 &   4827723 & 5392 & 4.52 &  0.08 & < 2.0 &    &     5460 &     4.60 &      P12 \\
  KOI-633 &   4841374 & 5732 & 4.09 & -0.24 & < 2.0 &    &     6074 &     4.03 &      P12 \\
  KOI-635 &   5020319 & 6111 & 4.40 & -0.01 &   5.8 &    &     6265 &     4.42 &      P12 \\
  KOI-638 &   5113822 & 5775 & 4.62 & -0.04 & < 2.0 &    &     5979 &     4.31 &      P12 \\
  KOI-639 &   5120087 & 6202 & 4.30 &  0.01 &   7.3 &    &     6431 &     4.42 &      P12 \\
  KOI-640 &   5121511 & 5265 & 4.40 &  0.10 & < 2.0 &    &     5256 &     4.50 &      P12 \\
  KOI-644 &   5356593 & 5749 & 4.25 & -0.17 & < 2.0 &    &     5688 &     3.80 &      P12 \\
  KOI-645 &   5374854 & 5821 & 4.15 & -0.30 & < 2.0 &    &     6307 &     4.09 &      P12 \\
  KOI-647 &   5531694 & 6065 & 4.12 & -0.48 &   2.6 &    &     6479 &     4.38 &      P12 \\
  KOI-649 &   5613330 & 6270 & 4.06 &  0.19 &   7.6 &    &     6288 &     4.29 &      P12 \\
  KOI-650 &   5786676 & 5043 & 4.43 &  0.01 & < 2.0 &    &     5096 &     4.55 &      P12 \\
  KOI-654 &   5941160 & 5784 & 4.48 & -0.08 & < 2.0 &    &     6035 &     4.24 &      P12 \\
  KOI-655 &   5966154 & 6151 & 4.18 & -0.09 & < 2.0 &    &     6465 &     4.39 &      P12 \\
  KOI-657 &   6020753 & 4769 & 4.51 & -0.24 & < 2.0 &    &     4763 &     4.63 &      P12 \\
  KOI-658 &   6062088 & 5917 & 4.47 &  0.03 & < 2.0 &    &     5924 &     4.52 &      P12 \\
  KOI-659 &   6125481 & 6312 & 4.29 & -0.10 &   8.6 &    &     6723 &     4.22 &      P12 \\
  KOI-660 &   6267535 & 5339 & 3.72 & -0.13 & < 2.0 &    &     5480 &     4.05 &      P12 \\
  KOI-661 &   6347299 & 5895 & 4.45 &  0.01 &   2.3 &    &     6098 &     4.40 &      P12 \\
  KOI-662 &   6365156 & 5800 & 4.01 & -0.08 & < 2.0 &    &     6148 &     4.41 &      P12 \\
  KOI-664 &   6442340 & 5728 & 4.34 &  0.02 & < 2.0 &    &     5986 &     4.24 &      P12 \\
  KOI-665 &   6685609 & 5933 & 4.06 &  0.25 &   4.9 &    &     6085 &     4.37 &      P12 \\
  KOI-666 &   6707835 & 5584 & 4.29 &  0.09 & < 2.0 &    &     5768 &     4.55 &      P12 \\
  KOI-670 &   7033671 & 5621 & 3.95 &  0.14 & < 2.0 &    &     5757 &     4.35 &      P12 \\
  KOI-671 &   7040629 & 6067 & 4.19 & -0.04 &   4.6 &    &     5780 &     4.44 &      Sol \\
  KOI-672 &   7115785 & 5502 & 4.34 &  0.06 & < 2.0 &    &     5758 &     4.16 &      P12 \\
  KOI-673 &   7124613 & 6317 & 4.28 & -0.02 &  12.7 &    &     6557 &     4.34 &      P12 \\
  KOI-674 &   7277317 & 4908 & 3.58 &  0.18 & < 2.0 &    &     4864 &     3.67 &      KIC \\
  KOI-678 &   7509886 & 5197 & 4.65 &  0.14 & < 2.0 &    &     5174 &     3.91 &      P12 \\
  KOI-679 &   7515212 & 5895 & 4.15 &  0.18 &   2.8 &    &     5780 &     4.44 &      Sol \\
  KOI-680 &   7529266 & 6202 & 4.01 & -0.02 &   6.0 &    &     6326 &     4.35 &      P12 \\
  KOI-682 &   7619236 & 5648 & 4.37 &  0.32 & < 2.0 &    &     5686 &     4.50 &      P12 \\
  KOI-683 &   7630229 & 5854 & 4.32 &  0.11 & < 2.0 &    &     5823 &     4.54 &      P12 \\
  KOI-684 &   7730747 & 5235 & 3.67 &  0.03 & < 2.0 &    &     5474 &     3.96 &      P12 \\
  KOI-685 &   7764367 & 6515 & 4.22 & -0.14 &  14.9 &    &     6348 &     4.16 &      P12 \\
  KOI-686 &   7906882 & 5641 & 4.25 & -0.04 & < 2.0 &    &     5558 &     4.47 &      P12 \\
  KOI-687 &   7976520 & 5894 & 4.41 &  0.03 &   3.8 &    &     5885 &     4.50 &      P12 \\
  KOI-688 &   8161561 & 6211 & 4.22 & -0.11 &   8.7 &    &     6464 &     4.25 &      P12 \\
  KOI-689 &   8361905 & 5379 & 4.22 & -0.52 & < 2.0 &    &     5438 &     4.60 &      KIC \\
  KOI-691 &   8480285 & 5889 & 4.09 & -0.41 & < 2.0 &    &     6277 &     4.34 &      P12 \\
  KOI-692 &   8557374 & 5744 & 4.39 &  0.16 & < 2.0 &    &     5793 &     4.55 &      P12 \\
  KOI-693 &   8738735 & 6022 & 4.10 & -0.09 &   5.8 &    &     6343 &     4.44 &      P12 \\
  KOI-694 &   8802165 & 5698 & 4.46 &  0.19 & < 2.0 &    &     5775 &     4.55 &      P12 \\
  KOI-695 &   8805348 & 5638 & 4.05 & -0.54 & < 2.0 &    &     6225 &     4.37 &      P12 \\
  KOI-697 &   8878187 & 5782 & 4.08 &  0.06 & < 2.0 &    &     5779 &     4.05 &      KIC \\
  KOI-700 &   8962094 & 5641 & 4.17 & -0.56 & < 2.0 &    &     5923 &     4.37 &      P12 \\
  KOI-701 &   9002278 & 4903 & 4.52 & -0.38 & < 2.0 &    &     5033 &     4.66 &      P12 \\
  KOI-703 &   9162741 & 6332 & 4.08 &  0.20 &   7.3 &    &     5780 &     4.44 &      Sol \\
  KOI-704 &   9266431 & 5319 & 4.59 & -0.10 & < 2.0 &    &     5444 &     4.47 &      P12 \\
  KOI-707 &   9458613 & 5980 & 4.10 &  0.09 &   3.9 &    &     6213 &     4.27 &      P12 \\
  KOI-708 &   9530945 & 6099 & 4.18 & -0.18 &   6.8 &    &     6279 &     4.45 &      P12 \\
  KOI-709 &   9578686 & 5302 & 4.28 & -0.23 & < 2.0 &    &     5658 &     4.52 &      P12 \\
  KOI-710 &   9590976 & 6466 & 4.16 & -0.16 &  14.9 &    &     5780 &     4.44 &      Sol \\
  KOI-711 &   9597345 & 5627 & 4.40 &  0.36 & < 2.0 &    &     5611 &     4.45 &      P12 \\
  KOI-712 &   9640976 & 5511 & 4.56 &  0.00 & < 2.0 &    &     5669 &     4.57 &      P12 \\
  KOI-714 &   9702072 & 5333 & 4.44 &  0.09 & < 2.0 &    &     5624 &     4.57 &      P12 \\
  KOI-717 &   9873254 & 5579 & 4.16 &  0.28 & < 2.0 &    &     5623 &     4.58 &      P12 \\
  KOI-718 &   9884104 & 5953 & 4.35 &  0.36 & < 2.0 &    &     6027 &     4.51 &      P12 \\
  KOI-719 &   9950612 & 4734 & 4.57 & -0.02 &   2.4 &    &     5780 &     4.44 &      Sol \\
  KOI-720 &   9963524 & 5264 & 4.67 & -0.02 &   4.0 &    &     5324 &     4.54 &      P12 \\
  KOI-721 &   9964801 & 5773 & 4.04 &  0.05 & < 2.0 &    &     6028 &     4.09 &      P12 \\
  KOI-722 &   9965439 & 6127 & 4.31 & -0.23 &   5.4 &    &     6294 &     4.45 &      P12 \\
  KOI-723 &  10002866 & 5332 & 4.65 &  0.28 &   3.2 &    &     5344 &     4.62 &      P12 \\
  KOI-730 &  10227020 & 5820 & 4.07 &  0.06 &   2.3 &    &     5833 &     4.39 &      P12 \\
  KOI-732 &  10265898 & 5204 & 4.36 &  0.23 & < 2.0 &    &     5379 &     4.59 &      P12 \\
  KOI-733 &  10271806 & 5065 & 4.60 & -0.20 & < 2.0 &    &     5217 &     4.64 &      P12 \\
  KOI-738 &  10358759 & 5366 & 4.26 & -0.57 & < 2.0 &    &     5969 &     4.52 &      P12 \\
  KOI-756 &  10872983 & 5672 & 4.19 &  0.09 & < 2.0 &    &     6011 &     4.51 &      P12 \\
  KOI-757 &  10910878 & 5042 & 4.62 & -0.01 & < 2.0 &    &     5101 &     4.65 &      P12 \\
  KOI-759 &  11018648 & 5244 & 4.38 & -0.29 & < 2.0 &    &     5608 &     4.56 &      P12 \\
  KOI-760 &  11138155 & 5712 & 4.35 & -0.00 & < 2.0 &    &     6080 &     4.50 &      P12 \\
  KOI-771 &  11465813 & 5638 & 4.25 &  0.04 &   2.3 &    &     6354 &     4.38 &      P12 \\
  KOI-806 &   3832474 & 5452 & 4.61 &  0.06 & < 2.0 &    &     5359 &     4.52 &      P12 \\
  KOI-825 &   5252423 & 4900 & 4.52 &  0.14 & < 2.0 &    &     4833 &     4.62 &      P12 \\
  KOI-834 &   5436502 & 5725 & 4.09 &  0.25 & < 2.0 &    &     5779 &     4.55 &      P12 \\
  KOI-835 &   5456651 & 4918 & 4.51 &  0.10 & < 2.0 &    &     4939 &     4.67 &      P12 \\
  KOI-841 &   5792202 & 5306 & 4.63 & -0.01 &   2.8 &    &     5333 &     4.62 &      P12 \\
  KOI-853 &   6428700 & 4885 & 4.63 & -0.09 &   2.2 &    &     4953 &     4.59 &      P12 \\
  KOI-857 &   6587280 & 5171 & 4.58 &  0.21 & < 2.0 &    &     5115 &     4.63 &      P12 \\
  KOI-864 &   6849310 & 5522 & 4.50 &  0.01 & < 2.0 &    &     5545 &     4.58 &      P12 \\
  KOI-869 &   6948054 & 5115 & 4.66 &  0.02 &   2.3 &    &     5221 &     4.52 &      P12 \\
  KOI-874 &   7134976 & 5106 & 4.60 &  0.14 & < 2.0 &    &     5122 &     4.55 &      P12 \\
  KOI-880 &   7366258 & 5429 & 4.40 &  0.13 & < 2.0 &    &     5701 &     4.49 &      P12 \\
  KOI-881 &   7373451 & 5086 & 4.57 & -0.09 & < 2.0 &    &     5213 &     4.64 &      P12 \\
  KOI-889 &    757450 & 5331 & 4.54 &  0.19 & < 2.0 &    &     5154 &     4.54 &      P12 \\
  KOI-896 &   7825899 & 5165 & 4.51 &  0.05 & < 2.0 &    &     5288 &     4.62 &      P12 \\
  KOI-907 &   8247638 & 5644 & 4.45 & -0.08 & < 2.0 &    &     5865 &     4.34 &      P12 \\
  KOI-918 &   8672910 & 5416 & 4.61 &  0.08 & < 2.0 &    &     5527 &     4.54 &      P12 \\
  KOI-934 &   9334289 & 5496 & 4.30 & -0.21 & < 2.0 &    &     5948 &     4.52 &      P12 \\
  KOI-935 &   9347899 & 6167 & 4.17 & -0.28 &   6.4 &    &     6503 &     4.40 &      P12 \\
  KOI-939 &   9466668 & 5618 & 4.34 &  0.19 & < 2.0 &    &     5865 &     4.54 &      P12 \\
  KOI-941 &   9480189 & 5134 & 4.60 &  0.32 & < 2.0 &    &     5063 &     4.56 &      P12 \\
  KOI-954 &   9823457 & 5505 & 4.36 & -0.17 & < 2.0 &    &     5927 &     4.53 &      P12 \\
  KOI-958 &   1026957 & 4914 & 4.61 & -0.04 & < 2.0 &    &     4917 &     4.60 &      P12 \\
  KOI-974 &   9414417 & 6277 & 4.08 & -0.10 &   7.6 &    &     6277 &     4.36 &      P12 \\
  KOI-975 &   3632418 & 6175 & 4.06 & -0.09 &   7.3 &    &     5780 &     4.44 &      Sol \\
  KOI-981 &   8607720 & 5021 & 3.08 & -0.24 &   2.6 &    &     5254 &     3.36 &      P12 \\
  KOI-986 &   2854698 & 5545 & 4.56 &  0.25 & < 2.0 &    &     5503 &     4.59 &      P12 \\
  KOI-987 &   7295235 & 5457 & 4.44 &  0.05 & < 2.0 &    &     5482 &     4.56 &      P12 \\
  KOI-988 &   2302548 & 5127 & 4.70 &  0.07 &   2.2 &    &     5161 &     3.88 &      P12 \\
  KOI-991 &  10154388 & 5494 & 4.31 & -0.22 & < 2.0 &    &     5939 &     4.07 &      P12 \\
 KOI-1001 &   1871056 & 6232 & 4.04 &  0.05 &   8.8 &    &     6235 &     3.80 &      P12 \\
 KOI-1002 &   1865042 & 5388 & 4.30 &  0.07 & < 2.0 &    &     5305 &     4.62 &      P12 \\
 KOI-1010 &   1027438 & 6119 & 4.15 & -0.10 &   7.0 &    &     6509 &     4.16 &      P12 \\
 KOI-1019 &   8179973 & 5023 & 3.51 &  0.12 &   2.1 &    &     4962 &     3.77 &      P12 \\
 KOI-1032 &   2162635 & 4902 & 3.38 & -0.05 &   2.4 &    &     4965 &     3.58 &      P12 \\
 KOI-1050 &   5809890 & 5064 & 4.52 &  0.05 & < 2.0 &    &     5097 &     4.55 &      P12 \\
 KOI-1052 &   5956342 & 5887 & 4.36 & -0.23 & < 2.0 &    &     6326 &     4.44 &      P12 \\
 KOI-1054 &   6032981 & 5350 & 2.57 & -0.92 &   5.5 &    &     5406 &     4.43 &      P12 \\
 KOI-1060 &   5880320 & 6266 & 4.11 & -0.46 &  12.3 &    &     6670 &     4.36 &      P12 \\
 KOI-1069 &   8222813 & 5188 & 4.46 &  0.21 & < 2.0 &    &     5221 &     4.31 &      KIC \\
 KOI-1089 &   3247268 & 5847 & 4.38 &  0.07 & < 2.0 &    &     6165 &     4.42 &      P12 \\
 KOI-1102 &   3231341 & 5805 & 4.25 & -0.40 &   5.5 &    &     6043 &     4.35 &      P12 \\
 KOI-1113 &   2854914 & 6108 & 4.25 & -0.01 &   5.0 &    &     6315 &     4.39 &      P12 \\
 KOI-1115 &   3116412 & 5673 & 4.03 &  0.08 & < 2.0 &    &     5685 &     4.22 &      P12 \\
 KOI-1116 &   2849805 & 5777 & 4.38 & -0.00 & < 2.0 &    &     6029 &     4.50 &      P12 \\
 KOI-1117 &   3114811 & 6406 & 4.05 & -0.09 &   9.5 &    &     6501 &     4.40 &      P12 \\
 KOI-1118 &   2853446 & 6017 & 4.20 & -0.11 &   2.7 &    &     6318 &     4.34 &      P12 \\
 KOI-1120 &   6307537 & 4944 & 3.51 &  0.09 &   3.5 &    &     5780 &     4.44 &      Sol \\
 KOI-1127 &   6359320 & 5658 & 4.17 &  0.33 & < 2.0 &    &     5602 &     4.56 &      KIC \\
 KOI-1128 &   6362874 & 5335 & 4.33 & -0.08 & < 2.0 &    &     5483 &     4.59 &      P12 \\
 KOI-1145 &   8313667 & 6008 & 4.38 &  0.03 &   2.4 &    &     6059 &     4.50 &      P12 \\
 KOI-1148 &   8410727 & 6110 & 4.25 &  0.11 &   4.5 &    &     6416 &     4.29 &      P12 \\
 KOI-1150 &   8278371 & 5807 & 4.36 &  0.07 &   2.4 &    &     5913 &     4.52 &      P12 \\
 KOI-1151 &   8280511 & 5466 & 4.31 & -0.25 & < 2.0 &    &     5757 &     4.43 &      P12 \\
 KOI-1161 &  10426656 & 5441 & 4.30 & -0.03 & < 2.0 &    &     5294 &     4.48 &      P12 \\
 KOI-1162 &  10528068 & 5645 & 3.95 & -0.31 & < 2.0 &    &     6139 &     4.28 &      P12 \\
 KOI-1165 &  10337517 & 5384 & 4.40 & -0.06 & < 2.0 &    &     5811 &     4.28 &      P12 \\
 KOI-1168 &  10460629 & 6121 & 4.10 & -0.01 &   6.3 &    &     6465 &     4.23 &      P12 \\
 KOI-1169 &  10319385 & 5662 & 4.29 &  0.11 & < 2.0 &    &     5957 &     4.52 &      P12 \\
 KOI-1175 &  10350571 & 5572 & 3.68 &  0.01 &   3.6 &    &     5650 &     4.57 &      P12 \\
 KOI-1198 &   3447722 & 6266 & 4.23 & -0.00 &   8.2 &    &     6474 &     4.41 &      P12 \\
 KOI-1199 &   3859079 & 4819 & 4.54 &  0.09 & < 2.0 &    &     4767 &     4.63 &      P12 \\
 KOI-1206 &   3756801 & 5756 & 3.83 &  0.03 &   5.0 &    &     5752 &     4.11 &      P12 \\
 KOI-1208 &   3962440 & 6277 & 4.11 & -0.20 &   8.0 &    &     6480 &     4.40 &      P12 \\
 KOI-1209 &   3534076 & 5819 & 4.44 &  0.01 & < 2.0 &    &     5588 &     4.58 &      P12 \\
 KOI-1215 &   3939150 & 6017 & 3.99 &  0.02 &   2.6 &    &     6049 &     4.23 &      P12 \\
 KOI-1216 &   3839488 & 5991 & 4.14 & -0.14 &   2.1 &    &     6120 &     4.33 &      P12 \\
 KOI-1218 &   3442055 & 5644 & 4.29 & -0.05 & < 2.0 &    &     5871 &     4.38 &      P12 \\
 KOI-1220 &   4043190 & 5302 & 3.76 &  0.11 & < 2.0 &    &     5167 &     4.53 &      P12 \\
 KOI-1221 &   3640905 & 4999 & 3.65 &  0.30 & < 2.0 &    &     5047 &     3.39 &      P12 \\
 KOI-1222 &   4060815 & 5088 & 3.47 &  0.01 & < 2.0 &    &     5019 &     4.57 &      P12 \\
 KOI-1230 &   6470149 & 5067 & 3.14 & -0.08 &   2.0 &    &     5103 &     3.00 &      P12 \\
 KOI-1239 &   6607286 & 5748 & 4.36 & -0.12 & < 2.0 &    &     5849 &     4.60 &      KIC \\
 KOI-1241 &   6448890 & 4894 & 3.40 &  0.37 & < 2.0 &    &     5004 &     3.22 &      P12 \\
 KOI-1242 &   6607447 & 6118 & 4.18 & -0.09 &   5.3 &    &     6441 &     4.42 &      P12 \\
 KOI-1257 &   8751933 & 5525 & 4.25 &  0.26 &   3.0 &    &     5315 &     4.47 &      P12 \\
 KOI-1271 &   8631160 & 6259 & 4.16 & -0.38 &   6.5 &    &     6630 &     4.23 &      P12 \\
 KOI-1274 &   8800954 & 5220 & 4.36 & -0.29 & < 2.0 &    &     5379 &     4.58 &      P12 \\
 KOI-1275 &   8583696 & 5822 & 4.23 & -0.04 & < 2.0 &    &     5626 &     4.44 &      P12 \\
 KOI-1276 &   8804283 & 5450 & 4.26 &  0.07 & < 2.0 &    &     5594 &     4.58 &      P12 \\
 KOI-1278 &   8609450 & 5615 & 3.86 & -0.34 & < 2.0 &    &     6141 &     4.48 &      P12 \\
 KOI-1279 &   8628758 & 5752 & 4.40 & -0.06 & < 2.0 &    &     5829 &     4.54 &      P12 \\
 KOI-1282 &   8822366 & 6017 & 4.11 & -0.25 &   6.1 &    &     6309 &     4.24 &      P12 \\
 KOI-1283 &   8700771 & 5669 & 3.75 & -0.38 & < 2.0 &    &     5780 &     4.44 &      Sol \\
 KOI-1288 &  10790387 & 6072 & 4.29 & -0.00 & < 2.0 &    &     6397 &     4.39 &      P12 \\
 KOI-1299 &  10864656 & 5002 & 3.34 &  0.02 &   2.0 &    &     5155 &     3.45 &      P12 \\
 KOI-1306 &  10858691 & 5529 & 4.11 & -0.40 & < 2.0 &    &     5973 &     4.51 &      P12 \\
 KOI-1308 &  10586208 & 5616 & 3.87 & -0.04 & < 2.0 &    &     5956 &     4.51 &      P12 \\
 KOI-1314 &  10585852 & 5073 & 3.52 &  0.06 & < 2.0 &    &     5186 &     3.70 &      P12 \\
 KOI-1315 &  10928043 & 6103 & 4.28 &  0.01 &   4.1 &    &     6417 &     4.31 &      P12 \\
 KOI-1316 &  10794087 & 5810 & 3.96 &  0.26 &   3.0 &    &     5780 &     4.44 &      Sol \\
 KOI-1335 &   4155328 & 6400 & 4.08 &  0.12 &  12.7 &    &     6221 &     4.04 &      P12 \\
 KOI-1336 &   4077526 & 5785 & 4.53 &  0.03 & < 2.0 &    &     6082 &     4.38 &      P12 \\
 KOI-1338 &   4466677 & 5643 & 4.09 & -0.26 & < 2.0 &    &     5835 &     4.43 &      P12 \\
 KOI-1344 &   4136466 & 6009 & 4.18 & -0.42 & < 2.0 &    &     6035 &     4.51 &      P12 \\
 KOI-1353 &   7303287 & 5995 & 4.55 & -0.04 &   5.4 &    &     6261 &     4.08 &      P12 \\
 KOI-1356 &   7363829 & 5677 & 3.82 &  0.11 &   3.0 &    &     5889 &     4.43 &      P12 \\
 KOI-1360 &   7102227 & 4894 & 4.44 & -0.27 & < 2.0 &    &     5117 &     4.65 &      P12 \\
 KOI-1363 &   6936909 & 5681 & 4.31 &  0.18 & < 2.0 &    &     5926 &     4.53 &      P12 \\
 KOI-1364 &   6962977 & 5299 & 4.42 & -0.01 & < 2.0 &    &     5446 &     4.47 &      P12 \\
 KOI-1366 &   6932987 & 5439 & 4.38 &  0.02 & < 2.0 &    &     5709 &     4.56 &      P12 \\
 KOI-1367 &   6934291 & 4947 & 4.53 & -0.18 & < 2.0 &    &     5070 &     4.64 &      P12 \\
 KOI-1375 &   6766634 & 6139 & 4.18 & -0.33 &   8.7 &    &     5780 &     4.44 &      Sol \\
 KOI-1378 &   7375795 & 5545 & 3.69 & -0.37 & < 2.0 &    &     5780 &     4.44 &      Sol \\
 KOI-1379 &   7211221 & 5723 & 4.38 & -0.12 & < 2.0 &    &     5868 &     4.54 &      P12 \\
 KOI-1396 &   9455556 & 5545 & 4.53 &  0.04 & < 2.0 &    &     5865 &     4.53 &      P12 \\
 KOI-1411 &   9425139 & 5679 & 4.25 &  0.33 & < 2.0 &    &     5472 &     4.40 &      P12 \\
 KOI-1412 &   8950853 & 5987 & 4.18 &  0.09 &   3.0 &    &     6211 &     4.41 &      P12 \\
 KOI-1413 &   9006449 & 5260 & 3.64 & -0.09 & < 2.0 &    &     5630 &     4.44 &      P12 \\
 KOI-1421 &  11342550 & 5650 & 4.27 & -0.05 & < 2.0 &    &     5852 &     4.45 &      P12 \\
 KOI-1426 &  11122894 & 5658 & 4.31 & -0.21 & < 2.0 &    &     6137 &     4.43 &      P12 \\
 KOI-1428 &  11401182 & 4812 & 4.51 & -0.19 & < 2.0 &    &     4855 &     4.61 &      P12 \\
 KOI-1431 &  11075279 & 5529 & 4.37 &  0.24 & < 2.0 &    &     5597 &     4.49 &      P12 \\
 KOI-1432 &  11014932 & 5650 & 4.26 &  0.02 & < 2.0 &    &     5884 &     4.53 &      P12 \\
 KOI-1436 &  11389771 & 5632 & 4.40 &  0.12 & < 2.0 &    &     5811 &     4.51 &      P12 \\
 KOI-1438 &  11193263 & 5747 & 4.06 &  0.15 &   2.5 &    &     5896 &     4.43 &      P12 \\
 KOI-1439 &  11027624 & 6000 & 4.05 &  0.10 &   5.0 &    &     6200 &     4.31 &      P12 \\
 KOI-1442 &  11600889 & 5610 & 4.40 &  0.43 & < 2.0 &    &     5569 &     4.33 &      P12 \\
 KOI-1444 &  11043167 & 6144 & 4.01 &  0.01 &   8.0 &    &     6372 &     4.23 &      P12 \\
 KOI-1445 &  11336883 & 6277 & 4.13 &  0.06 &  13.8 &    &     6532 &     4.36 &      P12 \\
 KOI-1463 &   7672940 & 6436 & 4.17 & -0.09 &  10.5 &    &     5780 &     4.44 &      Sol \\
 KOI-1466 &   9512981 & 4800 & 4.41 &  0.16 & < 2.0 &    &     4813 &     4.62 &      P12 \\
 KOI-1474 &  12365184 & 6378 & 4.13 &  0.13 &  13.6 &    &     6740 &     4.09 &      P12 \\
 KOI-1477 &   7811397 & 5283 & 4.61 & -0.10 & < 2.0 &    &     5475 &     4.60 &      P12 \\
 KOI-1478 &  12403119 & 5496 & 4.22 & -0.02 & < 2.0 &    &     5698 &     4.56 &      P12 \\
 KOI-1480 &   7512982 & 4928 & 4.52 & -0.32 &   2.0 &    &     5098 &     4.65 &      P12 \\
 KOI-1486 &   7898352 & 5746 & 4.37 &  0.10 & < 2.0 &    &     5952 &     4.52 &      P12 \\
 KOI-1528 &   7691260 & 5311 & 4.39 &  0.02 & < 2.0 &    &     5261 &     4.63 &      P12 \\
 KOI-1529 &   9821454 & 5828 & 4.18 & -0.33 & < 2.0 &    &     6308 &     4.45 &      P12 \\
 KOI-1530 &  11954842 & 5900 & 4.20 & -0.59 & < 2.0 &    &     6265 &     4.41 &      P12 \\
 KOI-1531 &  11764462 & 5860 & 4.46 & -0.09 & < 2.0 &    &     6069 &     4.40 &      P12 \\
 KOI-1532 &  11656246 & 6123 & 4.17 &  0.10 &   6.5 &    &     6447 &     4.29 &      P12 \\
 KOI-1533 &   7808587 & 5880 & 4.48 & -0.31 & < 2.0 &    &     6356 &     4.42 &      P12 \\
 KOI-1534 &   4741126 & 6204 & 4.21 & -0.02 &   7.8 &    &     6396 &     4.40 &      P12 \\
 KOI-1535 &  11669125 & 5738 & 4.43 & -0.42 & < 2.0 &    &     6189 &     4.33 &      P12 \\
 KOI-1536 &  12159249 & 5931 & 4.16 &  0.19 &   2.7 &    &     6057 &     4.40 &      P12 \\
 KOI-1537 &   9872292 & 6169 & 4.10 & -0.24 &   5.7 &    &     5780 &     4.44 &      Sol \\
 KOI-1546 &   5475431 & 6108 & 4.12 & -0.19 &   4.6 &    &     5615 &     4.58 &      P12 \\
 KOI-1557 &   5371776 & 4831 & 4.65 & -0.03 &   2.8 &    &     4789 &     4.62 &      P12 \\
 KOI-1563 &   5219234 & 5113 & 4.56 &  0.03 & < 2.0 &    &     4918 &     4.51 &      KIC \\
 KOI-1567 &   5438099 & 4886 & 4.29 & -0.22 & < 2.0 &    &     5027 &     4.52 &      KIC \\
 KOI-1576 &   5299459 & 5500 & 4.30 &  0.18 & < 2.0 &    &     5574 &     4.34 &      P12 \\
 KOI-1589 &   5301750 & 5970 & 4.50 & -0.25 &   4.2 &    &     6015 &     4.42 &      P12 \\
 KOI-1590 &   5542466 & 4818 & 4.41 & -0.22 &   2.6 &    &     4936 &     4.59 &      P12 \\
 KOI-1606 &   9886661 & 5443 & 4.51 &  0.10 & < 2.0 &    &     5548 &     4.57 &      P12 \\
 KOI-1608 &  10055126 & 5926 & 4.29 & -0.08 &   2.5 &    &     6284 &     4.38 &      P12 \\
 KOI-1609 &   5009743 & 5975 & 4.41 & -0.52 & < 2.0 &    &     6292 &     4.44 &      P12 \\
 KOI-1612 &  10963065 & 6019 & 4.23 & -0.24 &   2.8 &    &     6317 &     4.16 &      P12 \\
 KOI-1615 &   4278221 & 6049 & 4.44 &  0.19 &   7.4 &    &     5808 &     4.55 &      P12 \\
 KOI-1616 &   9015738 & 6034 & 4.26 &  0.12 &   4.8 &    &     5942 &     4.53 &      KIC \\
 KOI-1618 &   7215603 & 6203 & 4.14 &  0.08 &   9.7 &    &     6342 &     4.32 &      P12 \\
 KOI-1619 &   4276716 & 4871 & 4.53 & -0.30 & < 2.0 &    &     4827 &     4.62 &      P12 \\
 KOI-1621 &   5561278 & 6054 & 4.01 & -0.05 &   5.5 &    &     6218 &     4.33 &      P12 \\
 KOI-1623 &  11392618 & 5746 & 4.12 & -0.01 & < 2.0 &    &     5791 &     4.51 &      P12 \\
 KOI-1628 &   6975129 & 6212 & 4.40 &  0.09 &  10.3 &    &     6198 &     4.13 &      P12 \\
 KOI-1629 &   8685497 & 5798 & 4.19 &  0.23 &   2.2 &    &     5995 &     4.37 &      P12 \\
 KOI-1632 &   9277896 & 6091 & 4.10 & -0.03 &   7.1 &    &     6453 &     4.31 &      P12 \\
 KOI-1639 &  10749128 & 6035 & 3.75 &  0.01 &   5.5 &    &     6267 &     4.45 &      P12 \\
 KOI-1647 &  11153121 & 5756 & 4.28 &  0.25 & < 2.0 &    &     5881 &     4.36 &      P12 \\
 KOI-1655 &  11547505 & 5496 & 4.22 & -0.16 & < 2.0 &    &     5886 &     4.44 &      P12 \\
 KOI-1665 &   4932442 & 6017 & 4.18 &  0.30 & < 2.0 &    &     6100 &     4.49 &      P12 \\
 KOI-1666 &   5008501 & 6277 & 4.18 & -0.02 &  14.2 &    &     6419 &     4.42 &      P12 \\
 KOI-1669 &   5183357 & 6139 & 4.15 & -0.11 &   6.6 &    &     6382 &     4.42 &      P12 \\
 KOI-1688 &   6310636 & 6017 & 4.11 &  0.13 &   5.1 &    &     5821 &     4.50 &      P12 \\
 KOI-1692 &   6616218 & 5431 & 4.53 &  0.36 & < 2.0 &    &     5224 &     4.47 &      KIC \\
 KOI-1695 &   6803855 & 5907 & 4.17 &  0.09 & < 2.0 &    &     6127 &     4.15 &      P12 \\
 KOI-1706 &   7626370 & 5176 & 4.37 &  0.06 & < 2.0 &    &     5215 &     4.51 &      P12 \\
 KOI-1707 &   7703955 & 5620 & 4.00 & -0.39 & < 2.0 &    &     5774 &     4.50 &      P12 \\
 KOI-1715 &   9836959 & 5781 & 4.28 & -0.34 & < 2.0 &    &     6348 &     4.16 &      P12 \\
 KOI-1726 &   8242434 & 4782 & 4.44 &  0.06 & < 2.0 &    &     4734 &     4.64 &      P12 \\
 KOI-1738 &   4365645 & 5308 & 4.51 &  0.21 & < 2.0 &    &     5308 &     4.48 &      P12 \\
 KOI-1739 &   7199906 & 5802 & 4.22 & -0.02 & < 2.0 &    &     5969 &     4.52 &      P12 \\
 KOI-1751 &   9729691 & 5149 & 4.61 & -0.08 & < 2.0 &    &     5165 &     4.53 &      P12 \\
 KOI-1754 &   8651389 & 6194 & 4.30 & -0.10 &   6.5 &    &     5780 &     4.44 &      Sol \\
 KOI-1779 &   9909735 & 5833 & 4.59 &  0.27 &   6.7 &    &     5811 &     4.14 &      P12 \\
 KOI-1781 &  11551692 & 4925 & 4.68 &  0.16 &   3.9 &    &     4888 &     3.62 &      P12 \\
 KOI-1783 &  10005758 & 5969 & 4.32 &  0.08 & < 2.0 &    &     6235 &     4.46 &      P12 \\
 KOI-1792 &   8552719 & 5472 & 3.93 & -0.05 &   3.3 &    &     5288 &     4.58 &      P12 \\
 KOI-1796 &  10019399 & 6045 & 4.45 & -0.06 &   4.0 &    &     5780 &     4.44 &      Sol \\
 KOI-1797 &  10676014 & 4967 & 4.68 &  0.13 &   3.8 &    &     4909 &     4.60 &      P12 \\
 KOI-1800 &  11017901 & 5612 & 4.65 &  0.03 &   6.3 &    &     5601 &     4.43 &      P12 \\
 KOI-1802 &  11298298 & 5935 & 4.55 & -0.01 & < 2.0 &    &     6105 &     4.48 &      P12 \\
 KOI-1803 &   4349442 & 4937 & 4.63 &  0.01 & < 2.0 &    &     4932 &     4.59 &      P12 \\
 KOI-1805 &   4644952 & 5602 & 4.64 & -0.00 &   2.6 &    &     5704 &     4.08 &      P12 \\
 KOI-1806 &   9529744 & 6148 & 4.19 & -0.11 &   6.6 &    &     6435 &     4.41 &      P12 \\
 KOI-1808 &   7761918 & 6150 & 4.33 & -0.01 &   6.5 &    &     6278 &     4.35 &      P12 \\
 KOI-1809 &   8240797 & 5768 & 4.48 &  0.07 & < 2.0 &    &     5780 &     4.44 &      Sol \\
 KOI-1812 &   6279974 & 6011 & 4.26 & -0.07 & < 2.0 &    &     6284 &     4.42 &      P12 \\
 KOI-1813 &   9455325 & 5418 & 4.58 &  0.01 & < 2.0 &    &     5507 &     4.38 &      P12 \\
 KOI-1815 &   9872283 & 4811 & 4.64 &  0.06 & < 2.0 &    &     4742 &     4.63 &      P12 \\
 KOI-1818 &   7870032 & 5574 & 4.63 & -0.00 & < 2.0 &    &     5724 &     4.32 &      P12 \\
 KOI-1819 &   9597058 & 5451 & 4.66 & -0.00 & < 2.0 &    &     5482 &     4.60 &      P12 \\
 KOI-1820 &   8277797 & 5387 & 4.58 &  0.07 & < 2.0 &    &     5539 &     4.09 &      P12 \\
 KOI-1822 &   5124667 & 6026 & 4.37 & -0.32 &   4.1 &    &     6221 &     4.21 &      P12 \\
 KOI-1824 &   2989404 & 5965 & 4.32 & -0.26 & < 2.0 &    &     6252 &     4.21 &      P12 \\
 KOI-1825 &   5375194 & 5381 & 4.66 &  0.08 &   4.0 &    &     5548 &     4.06 &      P12 \\
 KOI-1826 &   6468138 & 5921 & 4.32 & -0.10 & < 2.0 &    &     6007 &     4.51 &      P12 \\
 KOI-1831 &  11601584 & 5219 & 4.40 &  0.12 & < 2.0 &    &     5322 &     4.62 &      P12 \\
 KOI-1835 &   9471268 & 5155 & 4.69 &  0.14 &   3.9 &    &     5124 &     3.89 &      P12 \\
 KOI-1837 &  10657406 & 5268 & 4.68 &  0.12 & < 2.0 &    &     5287 &     4.49 &      P12 \\
 KOI-1839 &   5856571 & 5459 & 4.59 &  0.07 &   6.9 &    &     5540 &     3.95 &      P12 \\
 KOI-1841 &  11760231 & 5196 & 4.57 &  0.00 & < 2.0 &    &     5228 &     4.51 &      P12 \\
 KOI-1848 &   7430034 & 5977 & 4.34 & -0.20 &   6.0 &    &     6272 &     4.44 &      P12 \\
 KOI-1850 &   8826168 & 5818 & 4.15 & -0.05 & < 2.0 &    &     5927 &     4.53 &      P12 \\
 KOI-1852 &   9763348 & 6277 & 4.14 & -0.31 &   3.1 &    &     5780 &     4.44 &      Sol \\
 KOI-1854 &   9662811 & 5551 & 4.33 & -0.02 & < 2.0 &    &     5601 &     4.15 &      P12 \\
 KOI-1856 &  11570749 & 5273 & 4.57 & -0.01 & < 2.0 &    &     5349 &     3.99 &      P12 \\
 KOI-1857 &  11297236 & 5835 & 4.47 & -0.04 & < 2.0 &    &     5861 &     4.53 &      P12 \\
 KOI-1858 &   8160953 & 5444 & 4.59 & -0.07 & < 2.0 &    &     5667 &     4.44 &      P12 \\
 KOI-1860 &   4157325 & 5725 & 4.50 &  0.09 & < 2.0 &    &     5708 &     4.37 &      KIC \\
 KOI-1861 &   3648437 & 6025 & 4.54 & -0.03 &   7.5 &    &     6166 &     4.48 &      P12 \\
 KOI-1862 &   7286173 & 5643 & 4.41 &  0.22 & < 2.0 &    &     5703 &     4.55 &      P12 \\
 KOI-1863 &  11126381 & 6017 & 4.42 &  0.19 &   3.6 &    &     6189 &     4.47 &      P12 \\
 KOI-1864 &   4149450 & 5599 & 3.89 &  0.07 & < 2.0 &    &     5801 &     3.85 &      P12 \\
 KOI-1875 &   9967771 & 5582 & 4.23 & -0.19 & < 2.0 &    &     5959 &     4.48 &      P12 \\
 KOI-1877 &  10454632 & 4907 & 4.60 & -0.01 & < 2.0 &    &     4949 &     3.75 &      P12 \\
 KOI-1878 &   3098810 & 6155 & 4.18 &  0.10 &   6.8 &    &     6248 &     4.35 &      P12 \\
 KOI-1883 &  11758544 & 6017 & 4.11 & -0.01 &   6.2 &    &     6294 &     4.34 &      P12 \\
 KOI-1886 &   9549648 & 6188 & 4.10 & -0.02 &  10.2 &    &     6345 &     4.02 &      P12 \\
 KOI-1888 &  10063802 & 6359 & 4.14 &  0.02 &  16.9 &    &     6739 &     4.25 &      P12 \\
 KOI-1889 &  11074178 & 5438 & 4.56 & -0.02 & < 2.0 &    &     5733 &     4.56 &      P12 \\
 KOI-1890 &   7449136 & 6087 & 4.12 &  0.05 &   6.9 &    &     6169 &     4.34 &      P12 \\
 KOI-1893 &   8689793 & 5742 & 4.17 & -0.34 & < 2.0 &    &     6112 &     4.49 &      P12 \\
 KOI-1894 &  11673802 & 5013 & 3.49 &  0.13 & < 2.0 &    &     4999 &     2.87 &      P12 \\
 KOI-1897 &   5695524 & 5851 & 4.25 & -0.20 & < 2.0 &    &     6190 &     4.39 &      P12 \\
 KOI-1898 &   7668663 & 5725 & 4.30 & -0.04 & < 2.0 &    &     6056 &     4.41 &      P12 \\
 KOI-1901 &   3629967 & 6017 & 4.29 &  0.10 &   3.7 &    &     6074 &     4.50 &      P12 \\
 KOI-1904 &   8766650 & 5076 & 4.58 & -0.04 & < 2.0 &    &     5059 &     3.85 &      P12 \\
 KOI-1905 &  10328393 & 4936 & 4.56 & -0.18 & < 2.0 &    &     5072 &     4.56 &      P12 \\
 KOI-1909 &  10130039 & 5895 & 4.45 & -0.03 & < 2.0 &    &     6095 &     4.46 &      P12 \\
 KOI-1913 &   9704384 & 5498 & 4.54 &  0.19 & < 2.0 &    &     5517 &     4.41 &      P12 \\
 KOI-1915 &   9101496 & 6011 & 4.08 &  0.31 &   5.8 &    &     5993 &     4.51 &      P12 \\
 KOI-1916 &   6037581 & 5913 & 4.40 &  0.20 &   5.2 &    &     6063 &     4.50 &      P12 \\
 KOI-1917 &  10074466 & 5983 & 4.32 & -0.11 &   2.5 &    &     6356 &     4.42 &      P12 \\
 KOI-1921 &   7755636 & 6387 & 4.16 & -0.06 &  18.6 &    &     6716 &     4.29 &      P12 \\
 KOI-1923 &   4989057 & 5391 & 4.44 &  0.15 & < 2.0 &    &     5453 &     4.04 &      P12 \\
 KOI-1924 &   5108214 & 5991 & 3.92 &  0.34 &   4.7 &    &     5911 &     3.86 &      P12 \\
 KOI-1925 &   9955598 & 5441 & 4.43 &  0.10 & < 2.0 &    &     5432 &     3.71 &      P12 \\
 KOI-1928 &   5770074 & 5900 & 4.43 &  0.22 &   2.1 &    &     6000 &     4.48 &      P12 \\
 KOI-1929 &  10136549 & 5651 & 3.89 &  0.02 & < 2.0 &    &     5900 &     4.12 &      P12 \\
 KOI-1930 &   5511081 & 5887 & 4.01 & -0.08 &   4.6 &    &     6164 &     4.06 &      P12 \\
 KOI-1938 &   9651234 & 5096 & 4.37 & -0.29 & < 2.0 &    &     5268 &     4.63 &      P12 \\
 KOI-1944 &   2438513 & 5760 & 4.68 &  0.03 & < 2.0 &    &     6287 &     3.98 &      P12 \\
 KOI-1947 &  12253474 & 5978 & 4.01 &  0.20 & < 2.0 &    &     6085 &     4.45 &      P12 \\
 KOI-1951 &   8081187 & 6017 & 4.21 & -0.31 &   4.0 &    &     6290 &     4.44 &      P12 \\
 KOI-1955 &   9892816 & 6214 & 4.15 &  0.02 &   9.3 &    &     6456 &     4.41 &      P12 \\
 KOI-1958 &   9836149 & 5872 & 4.64 & -0.00 &   3.6 &    &     5959 &     4.52 &      P12 \\
 KOI-1960 &   6949061 & 5805 & 4.25 &  0.13 &   2.2 &    &     6114 &     4.41 &      P12 \\
 KOI-1961 &   7269493 & 5408 & 4.59 & -0.01 &   2.9 &    &     5539 &     3.95 &      P12 \\
 KOI-1962 &   5513648 & 5941 & 4.13 & -0.09 &   3.8 &    &     5780 &     4.44 &      Sol \\
 KOI-1963 &  10917681 & 5856 & 4.22 &  0.03 &   3.6 &    &     6074 &     4.49 &      P12 \\
 KOI-1964 &   7887791 & 5545 & 4.39 &  0.00 & < 2.0 &    &     5541 &     3.83 &      P12 \\
 KOI-1978 &   9518318 & 5491 & 4.43 &  0.03 & < 2.0 &    &     5995 &     4.48 &      P12 \\
 KOI-1979 &   7273277 & 5756 & 4.37 &  0.16 & < 2.0 &    &     5794 &     4.47 &      P12 \\
 KOI-1980 &  11769890 & 5504 & 4.59 &  0.15 & < 2.0 &    &     5587 &     4.57 &      P12 \\
 KOI-1984 &  10094670 & 6017 & 4.34 &  0.08 &   3.2 &    &     6163 &     4.48 &      P12 \\
 KOI-1985 &   8142942 & 4934 & 4.61 & -0.03 & < 2.0 &    &     4930 &     4.59 &      P12 \\
 KOI-1989 &  10779233 & 5711 & 4.56 &  0.04 & < 2.0 &    &     5794 &     4.29 &      P12 \\
 KOI-2001 &   6061773 & 5158 & 4.64 &  0.03 &   2.8 &    &     5121 &     3.89 &      P12 \\
 KOI-2002 &  10024701 & 5998 & 4.43 & -0.03 &   4.0 &    &     5991 &     4.51 &      P12 \\
 KOI-2004 &  12154526 & 5719 & 4.36 &  0.29 &   3.7 &    &     5762 &     4.47 &      P12 \\
 KOI-2007 &  11069176 & 5911 & 4.54 &  0.09 & < 2.0 &    &     6063 &     4.41 &      P12 \\
 KOI-2009 &   2449431 & 5603 & 4.04 & -0.32 & < 2.0 &    &     5892 &     4.46 &      P12 \\
 KOI-2010 &   5631630 & 6392 & 4.18 & -0.06 &   9.8 &    &     6798 &     4.31 &      P12 \\
 KOI-2011 &   5384079 & 6345 & 4.22 & -0.13 &  15.2 &    &     6360 &     4.43 &      P12 \\
 KOI-2016 &   8492026 & 5885 & 4.17 &  0.30 &   2.6 &    &     5866 &     4.55 &      KIC \\
 KOI-2017 &   8750043 & 5679 & 4.60 & -0.00 &   2.6 &    &     5782 &     4.52 &      P12 \\
 KOI-2026 &  11923284 & 6017 & 4.53 & -0.17 &   3.7 &    &     6421 &     4.28 &      P12 \\
 KOI-2029 &   9489524 & 5225 & 4.67 & -0.19 & < 2.0 &    &     5225 &     4.63 &      P12 \\
 KOI-2033 &   2304320 & 5066 & 4.42 & -0.17 & < 2.0 &    &     5177 &     4.64 &      P12 \\
 KOI-2035 &   9790806 & 5569 & 4.66 &  0.05 &   5.6 &    &     5653 &     4.29 &      P12 \\
 KOI-2037 &   9634821 & 4903 & 4.66 &  0.16 &   2.9 &    &     4836 &     4.30 &      KIC \\
 KOI-2038 &   8950568 & 5533 & 4.58 &  0.05 & < 2.0 &    &     5667 &     4.57 &      P12 \\
 KOI-2039 &   8804845 & 5570 & 4.65 &  0.21 & < 2.0 &    &     5597 &     4.58 &      P12 \\
 KOI-2040 &  10480915 & 5599 & 4.16 & -0.05 & < 2.0 &    &     6004 &     4.51 &      P12 \\
 KOI-2043 &   3448130 & 5837 & 4.28 & -0.05 & < 2.0 &    &     6005 &     4.51 &      P12 \\
 KOI-2044 &   9656252 & 5674 & 4.42 &  0.12 & < 2.0 &    &     5805 &     4.51 &      KIC \\
 KOI-2046 &  10663396 & 5585 & 3.99 &  0.18 & < 2.0 &    &     5556 &     4.29 &      KIC \\
 KOI-2047 &  11457726 & 6156 & 4.31 & -0.09 &   4.6 &    &     6579 &     4.33 &      P12 \\
 KOI-2048 &   8956206 & 5168 & 4.63 &  0.05 & < 2.0 &    &     5156 &     4.64 &      P12 \\
 KOI-2049 &   9649706 & 5992 & 4.18 &  0.02 &   3.1 &    &     6292 &     4.43 &      P12 \\
 KOI-2051 &   7265298 & 5786 & 4.30 & -0.10 & < 2.0 &    &     5929 &     4.45 &      KIC \\
 KOI-2053 &   2307415 & 6091 & 4.13 & -0.01 &   6.6 &    &     6317 &     4.34 &      P12 \\
 KOI-2071 &   6035124 & 5236 & 4.41 &  0.12 & < 2.0 &    &     5409 &     4.01 &      P12 \\
 KOI-2072 &  12058147 & 5855 & 4.20 & -0.22 & < 2.0 &    &     6123 &     4.48 &      P12 \\
 KOI-2079 &   9473078 & 5458 & 4.38 &  0.38 & < 2.0 &    &     5436 &     4.42 &      P12 \\
 KOI-2081 &   2853780 & 5077 & 3.56 &  0.12 & < 2.0 &    &     5250 &     3.60 &      P12 \\
 KOI-2082 &   9472000 & 6017 & 4.21 &  0.30 &   2.1 &    &     6061 &     4.50 &      P12 \\
 KOI-2083 &   7097965 & 6071 & 4.36 & -0.08 &   5.2 &    &     6240 &     4.29 &      P12 \\
 KOI-2086 &   6768394 & 5861 & 4.11 & -0.09 & < 2.0 &    &     6177 &     4.16 &      P12 \\
 KOI-2087 &   6922710 & 5998 & 4.46 & -0.02 & < 2.0 &    &     6226 &     4.27 &      P12 \\
 KOI-2093 &   6525946 & 5990 & 4.36 & -0.04 &   3.2 &    &     6287 &     4.50 &      KIC \\
 KOI-2098 &   6105462 & 6266 & 4.22 & -0.23 &  11.3 &    &     6451 &     4.23 &      P12 \\
 KOI-2105 &   8165946 & 5927 & 4.40 & -0.11 &   2.2 &    &     6201 &     4.46 &      P12 \\
 KOI-2109 &  11499228 & 6021 & 4.06 & -0.03 &   7.0 &    &     6286 &     4.44 &      P12 \\
 KOI-2110 &  11460462 & 6329 & 4.17 &  0.16 &  16.4 &    &     6467 &     4.31 &      P12 \\
 KOI-2111 &   8612275 & 5643 & 4.60 &  0.11 &   3.3 &    &     6036 &     4.42 &      P12 \\
 KOI-2115 &   9532052 & 5267 & 4.71 & -0.00 & < 2.0 &    &     5184 &     4.45 &      KIC \\
 KOI-2119 &   4055304 & 5121 & 4.63 &  0.14 &   2.3 &    &     5100 &     4.55 &      P12 \\
 KOI-2120 &   4857213 & 5065 & 4.64 & -0.09 & < 2.0 &    &     5064 &     3.85 &      P12 \\
 KOI-2133 &   8219268 & 4644 & 2.91 &  0.34 &   3.6 &    &     4837 &     2.85 &      P12 \\
 KOI-2135 &   9904006 & 6109 & 4.10 & -0.03 &   7.4 &    &     6320 &     4.31 &      P12 \\
 KOI-2137 &   9364609 & 5235 & 4.35 & -0.22 & < 2.0 &    &     5468 &     4.04 &      P12 \\
 KOI-2143 &  11403339 & 5440 & 4.51 &  0.18 & < 2.0 &    &     5552 &     4.58 &      P12 \\
 KOI-2148 &   6021193 & 5712 & 4.14 &  0.45 & < 2.0 &    &     5602 &     3.90 &      P12 \\
 KOI-2149 &  10617017 & 6217 & 4.16 &  0.17 &   8.6 &    &     6314 &     4.20 &      P12 \\
 KOI-2153 &  10253547 & 6033 & 4.14 & -0.11 &   5.5 &    &     6503 &     4.39 &      P12 \\
 KOI-2158 &   5211199 & 5387 & 4.28 & -0.02 & < 2.0 &    &     5412 &     4.02 &      P12 \\
 KOI-2159 &   8804455 & 5739 & 4.47 &  0.07 & < 2.0 &    &     5848 &     4.54 &      P12 \\
 KOI-2162 &   9205938 & 5664 & 4.21 & -0.53 & < 2.0 &    &     6145 &     4.48 &      P12 \\
 KOI-2168 &  11308499 & 5971 & 4.28 & -0.13 &   3.1 &    &     6185 &     4.47 &      P12 \\
 KOI-2169 &   9006186 & 5422 & 4.59 &  0.15 & < 2.0 &    &     5444 &     4.42 &      P12 \\
 KOI-2173 &  11774991 & 4847 & 4.66 &  0.08 &   2.0 &    &     4738 &     4.64 &      P12 \\
 KOI-2175 &   9022166 & 5463 & 3.87 &  0.07 & < 2.0 &    &     5293 &     4.58 &      KIC \\
 KOI-2188 &  10518424 & 5600 & 3.88 & -0.78 & < 2.0 &    &     6133 &     4.48 &      P12 \\
 KOI-2194 &   3548044 & 5749 & 4.18 & -0.29 & < 2.0 &    &     6036 &     4.51 &      P12 \\
 KOI-2201 &   2141783 & 6038 & 4.06 &  0.13 &   7.2 &    &     6083 &     4.30 &      P12 \\
 KOI-2202 &   4144576 & 5318 & 4.58 &  0.31 & < 2.0 &    &     5252 &     4.63 &      P12 \\
 KOI-2208 &  10531955 & 5863 & 4.30 &  0.06 & < 2.0 &    &     5780 &     4.44 &      Sol \\
 KOI-2218 &  12058204 & 5581 & 4.37 &  0.04 &   2.5 &    &     5803 &     4.55 &      P12 \\
 KOI-2219 &   5357545 & 4999 & 4.55 &  0.10 & < 2.0 &    &     4969 &     4.63 &      P12 \\
 KOI-2228 &  10801100 & 6480 & 4.16 & -0.26 &  12.6 &    &     5780 &     4.44 &      Sol \\
 KOI-2246 &   9458343 & 5667 & 4.26 & -0.27 & < 2.0 &    &     6057 &     4.50 &      P12 \\
 KOI-2248 &  11030475 & 5190 & 4.63 &  0.02 & < 2.0 &    &     5293 &     4.61 &      P12 \\
 KOI-2250 &   5942808 & 4946 & 4.61 &  0.04 &   2.5 &    &     4749 &     4.49 &      KIC \\
 KOI-2252 &   6206214 & 6117 & 3.99 &  0.03 &   7.3 &    &     6371 &     4.27 &      P12 \\
 KOI-2260 &  11811193 & 6169 & 4.17 & -0.05 &   7.4 &    &     6436 &     4.41 &      P12 \\
 KOI-2261 &   3734418 & 5172 & 4.65 &  0.01 & < 2.0 &    &     5176 &     4.53 &      P12 \\
 KOI-2273 &   9717943 & 6040 & 4.26 &  0.20 &   4.3 &    &     6162 &     4.31 &      P12 \\
 KOI-2278 &   3342794 & 5818 & 4.09 & -0.23 & < 2.0 &    &     6345 &     4.37 &      P12 \\
 KOI-2279 &   3661886 & 5952 & 4.27 & -0.00 & < 2.0 &    &     6204 &     4.47 &      P12 \\
 KOI-2281 &   9221517 & 5041 & 4.46 &  0.12 & < 2.0 &    &     5089 &     4.57 &      P12 \\
 KOI-2289 &   3867615 & 6017 & 4.23 &  0.02 &   3.8 &    &     6255 &     4.38 &      P12 \\
 KOI-2290 &  12121570 & 5005 & 4.54 & -0.31 & < 2.0 &    &     5122 &     4.65 &      P12 \\
 KOI-2295 &   4049901 & 5415 & 4.35 & -0.21 &   3.5 &    &     5451 &     4.45 &      P12 \\
 KOI-2300 &  10583761 & 5106 & 4.45 & -0.19 & < 2.0 &    &     5263 &     4.50 &      P12 \\
 KOI-2312 &  10026544 & 6235 & 4.07 & -0.38 &   6.1 &    &     6263 &     4.45 &      P12 \\
 KOI-2319 &   9003401 & 6061 & 4.22 & -0.10 &   4.3 &    &     6483 &     4.33 &      P12 \\
 KOI-2331 &  12401863 & 5835 & 4.16 &  0.04 & < 2.0 &    &     6048 &     4.41 &      P12 \\
 KOI-2332 &   5534941 & 5194 & 3.63 & -0.09 & < 2.0 &    &     5435 &     4.01 &      P12 \\
 KOI-2333 &  11121752 & 6017 & 4.27 & -0.26 &   3.5 &    &     6190 &     4.23 &      P12 \\
 KOI-2335 &   2990873 & 5568 & 4.31 & -0.05 & < 2.0 &    &     5859 &     4.30 &      P12 \\
 KOI-2342 &  10212441 & 5848 & 4.21 & -0.51 & < 2.0 &    &     6171 &     4.30 &      P12 \\
 KOI-2352 &   8013439 & 6277 & 4.17 & -0.28 &   6.7 &    &     5780 &     4.44 &      Sol \\
 KOI-2358 &   5716932 & 6253 & 4.12 &  0.15 &  13.5 &    &     6424 &     4.42 &      P12 \\
 KOI-2365 &  11560897 & 5985 & 4.21 &  0.18 &   2.7 &    &     6242 &     4.35 &      P12 \\
 KOI-2366 &  11342416 & 6145 & 4.21 & -0.05 &   6.1 &    &     6329 &     4.32 &      P12 \\
 KOI-2367 &   9086251 & 6039 & 4.10 &  0.09 &   6.1 &    &     6292 &     4.35 &      P12 \\
 KOI-2369 &   5602588 & 5802 & 4.20 &  0.04 & < 2.0 &    &     6048 &     4.50 &      P12 \\
 KOI-2370 &   5385304 & 6406 & 4.34 & -0.25 &  19.2 &    &     6710 &     4.19 &      P12 \\
 KOI-2372 &  12254909 & 6015 & 4.15 & -0.12 &   3.9 &    &     6217 &     4.44 &      P12 \\
 KOI-2389 &   8494617 & 5868 & 4.13 & -0.12 & < 2.0 &    &     6283 &     4.32 &      P12 \\
 KOI-2390 &  10289119 & 5960 & 3.95 &  0.07 &   4.8 &    &     6052 &     4.29 &      P12 \\
 KOI-2393 &   4665571 & 4879 & 4.57 & -0.11 & < 2.0 &    &     4899 &     4.61 &      P12 \\
 KOI-2396 &  12115188 & 5245 & 4.54 &  0.06 & < 2.0 &    &     5441 &     4.46 &      P12 \\
 KOI-2398 &   6199056 & 6095 & 4.13 & -0.42 &   8.0 &    &     6538 &     4.18 &      P12 \\
 KOI-2399 &  11461433 & 5099 & 4.57 & -0.09 & < 2.0 &    &     5216 &     4.63 &      P12 \\
 KOI-2403 &   2142522 & 6134 & 4.30 &  0.11 &   5.2 &    &     6294 &     4.42 &      P12 \\
 KOI-2407 &  12120484 & 5979 & 4.15 &  0.15 &   4.6 &    &     6195 &     4.47 &      P12 \\
 KOI-2408 &   6429812 & 5477 & 4.34 & -0.12 & < 2.0 &    &     5842 &     4.44 &      P12 \\
 KOI-2409 &  10024051 & 4807 & 4.15 & -0.68 & < 2.0 &    &     5285 &     4.62 &      P12 \\
 KOI-2410 &   8676038 & 5550 & 4.10 & -0.25 & < 2.0 &    &     6034 &     4.50 &      P12 \\
 KOI-2414 &   8611832 & 5505 & 3.67 & -0.40 & < 2.0 &    &     5888 &     4.51 &      P12 \\
 KOI-2422 &  11360805 & 5248 & 4.53 & -0.07 & < 2.0 &    &     5412 &     4.43 &      P12 \\
 KOI-2426 &   8081899 & 5330 & 4.21 &  0.03 & < 2.0 &    &     5449 &     4.60 &      P12 \\
 KOI-2433 &  11968463 & 5861 & 4.19 & -0.07 & < 2.0 &    &     6084 &     4.44 &      KIC \\
 KOI-2440 &   5339567 & 5699 & 4.20 &  0.32 & < 2.0 &    &     5656 &     4.42 &      P12 \\
 KOI-2443 &   9209624 & 5765 & 4.24 & -0.42 & < 2.0 &    &     6315 &     4.42 &      P12 \\
 KOI-2462 &   5042210 & 6017 & 4.05 &  0.03 &   5.1 &    &     6049 &     4.16 &      P12 \\
 KOI-2463 &  12454461 & 6047 & 4.22 &  0.14 &   5.2 &    &     6097 &     4.49 &      P12 \\
 KOI-2469 &   6149910 & 4836 & 4.52 & -0.17 & < 2.0 &    &     4833 &     4.62 &      P12 \\
 KOI-2470 &   9108085 & 5859 & 4.22 &  0.27 & < 2.0 &    &     5717 &     4.56 &      P12 \\
 KOI-2474 &   8240617 & 5367 & 4.53 & -0.32 & < 2.0 &    &     5522 &     4.59 &      P12 \\
 KOI-2479 &   5963582 & 5381 & 3.82 &  0.01 & < 2.0 &    &     5492 &     3.97 &      P12 \\
 KOI-2481 &   4476423 & 4752 & 2.94 &  0.08 &   3.2 &    &     4982 &     3.02 &      P12 \\
 KOI-2484 &  10453588 & 5736 & 4.12 & -0.41 & < 2.0 &    &     6046 &     4.37 &      P12 \\
 KOI-2486 &   8074328 & 6024 & 4.17 &  0.04 &   5.4 &    &     5780 &     4.44 &      Sol \\
 KOI-2488 &   8559152 & 5976 & 4.11 & -0.08 &   3.8 &    &     6441 &     4.28 &      P12 \\
 KOI-2492 &  11752632 & 5664 & 3.95 & -0.39 & < 2.0 &    &     6064 &     4.50 &      P12 \\
 KOI-2498 &   5959719 & 5170 & 4.40 & -0.12 & < 2.0 &    &     5309 &     4.61 &      P12 \\
 KOI-2503 &   8631504 & 4868 & 4.46 &  0.13 & < 2.0 &    &     4916 &     3.70 &      P12 \\
 KOI-2516 &   7294743 & 5448 & 3.95 &  0.25 & < 2.0 &    &     5450 &     3.97 &      P12 \\
 KOI-2517 &   8947520 & 5582 & 4.45 & -0.17 & < 2.0 &    &     5943 &     4.44 &      P12 \\
 KOI-2521 &   7183745 & 4949 & 4.39 & -0.36 & < 2.0 &    &     5085 &     4.72 &      KIC \\
 KOI-2522 &   9177629 & 4938 & 4.56 &  0.19 & < 2.0 &    &     4847 &     4.61 &      P12 \\
 KOI-2530 &   9011825 & 5917 & 4.04 &  0.08 &   4.2 &    &     6115 &     4.38 &      P12 \\
 KOI-2533 &  11074835 & 5031 & 3.54 & -0.01 &   2.6 &    &     5173 &     3.61 &      P12 \\
 KOI-2534 &   1996180 & 6131 & 4.33 & -0.03 &   4.1 &    &     6176 &     4.46 &      P12 \\
 KOI-2538 &   1849702 & 5006 & 4.46 & -0.28 &   6.2 &    &     5176 &     4.64 &      P12 \\
 KOI-2541 &  12306058 & 5056 & 3.61 &  0.07 & < 2.0 &    &     5213 &     3.74 &      P12 \\
 KOI-2545 &   9696358 & 6042 & 3.92 &  0.06 &   6.6 &    &     6319 &     4.30 &      P12 \\
 KOI-2547 &   4484336 & 5890 & 4.27 & -0.23 & < 2.0 &    &     6137 &     4.37 &      P12 \\
 KOI-2555 &   5350244 & 6176 & 4.32 & -0.11 &   5.9 &    &     6481 &     4.36 &      P12 \\
 KOI-2556 &   5374403 & 5457 & 4.27 & -0.25 & < 2.0 &    &     5743 &     4.55 &      P12 \\
 KOI-2559 &   6605493 & 5848 & 4.32 &  0.08 & < 2.0 &    &     6122 &     4.48 &      P12 \\
 KOI-2561 &   7259298 & 6017 & 4.15 & -0.01 &   2.9 &    &     6106 &     4.49 &      P12 \\
 KOI-2563 &   5175024 & 6069 & 3.95 &  0.03 &   7.4 &    &     6386 &     4.37 &      P12 \\
 KOI-2564 &   9026749 & 6017 & 3.97 & -0.25 &   8.9 &    &     6259 &     4.45 &      P12 \\
 KOI-2571 &   6867588 & 5323 & 4.60 &  0.24 &   5.5 &    &     5160 &     4.64 &      P12 \\
 KOI-2581 &  11818872 & 5473 & 4.42 &  0.24 & < 2.0 &    &     5599 &     4.58 &      P12 \\
 KOI-2582 &  11771430 & 5887 & 4.20 &  0.28 & < 2.0 &    &     6124 &     4.41 &      P12 \\
 KOI-2583 &  10387742 & 5496 & 4.16 &  0.03 & < 2.0 &    &     5740 &     4.49 &      P12 \\
 KOI-2585 &   7673841 & 5866 & 4.23 & -0.50 & < 2.0 &    &     6484 &     4.20 &      P12 \\
 KOI-2590 &  12016267 & 6165 & 4.02 & -0.07 &  10.0 &    &     6435 &     4.07 &      P12 \\
 KOI-2593 &   8212002 & 6156 & 4.16 &  0.13 &   7.1 &    &     5780 &     4.44 &      Sol \\
 KOI-2595 &   8883329 & 6289 & 4.18 & -0.03 &  14.4 &    &     6740 &     4.11 &      P12 \\
 KOI-2597 &  12120307 & 5875 & 4.42 & -0.40 & < 2.0 &    &     6395 &     4.42 &      P12 \\
 KOI-2603 &   2443393 & 6277 & 4.17 & -0.13 &   9.2 &    &     5780 &     4.44 &      Sol \\
 KOI-2607 &   5095635 & 5762 & 4.49 &  0.14 & < 2.0 &    &     5884 &     4.53 &      P12 \\
 KOI-2608 &   6269070 & 6389 & 4.25 & -0.02 &  18.1 &    &     5780 &     4.44 &      Sol \\
 KOI-2612 &   9602613 & 5547 & 4.33 &  0.27 & < 2.0 &    &     5452 &     4.43 &      P12 \\
 KOI-2623 &  10916600 & 6188 & 4.07 &  0.07 &   6.8 &    &     6541 &     4.38 &      P12 \\
 KOI-2631 &   7584650 & 5756 & 4.11 & -0.52 & < 2.0 &    &     6131 &     4.31 &      P12 \\
 KOI-2632 &  11337566 & 6208 & 4.01 & -0.08 &  10.1 &    &     6461 &     4.20 &      P12 \\
 KOI-2635 &   4914566 & 6017 & 4.06 & -0.24 &   6.5 &    &     6266 &     4.22 &      P12 \\
 KOI-2636 &   6198182 & 5900 & 4.49 &  0.04 &   2.3 &    &     5780 &     4.44 &      Sol \\
 KOI-2639 &  11391755 & 5659 & 3.90 & -0.05 & < 2.0 &    &     6096 &     4.36 &      P12 \\
 KOI-2640 &   9088780 & 4909 & 2.88 & -0.24 &   2.4 &    &     4860 &     3.35 &      KIC \\
 KOI-2641 &   8894646 & 5847 & 4.14 & -0.03 & < 2.0 &    &     5834 &     4.33 &      P12 \\
 KOI-2657 &   9283156 & 5404 & 4.25 & -0.24 & < 2.0 &    &     5540 &     4.59 &      P12 \\
 KOI-2659 &   8803882 & 5029 & 3.51 &  0.17 & < 2.0 &    &     5190 &     3.51 &      P12 \\
 KOI-2668 &   5513012 & 5545 & 4.59 & -0.04 & < 2.0 &    &     5610 &     4.58 &      P12 \\
 KOI-2672 &  11253827 & 5696 & 4.63 &  0.16 &   2.7 &    &     5568 &     4.33 &      P12 \\
 KOI-2674 &   8022489 & 5732 & 4.10 &  0.04 & < 2.0 &    &     5972 &     4.26 &      P12 \\
 KOI-2675 &   5794570 & 5740 & 4.69 &  0.07 &   7.3 &    &     5697 &     4.56 &      P12 \\
 KOI-2676 &   5649325 & 6272 & 3.99 & -0.13 &   3.8 &    &     5954 &     3.83 &      P12 \\
 KOI-2677 &   9958387 & 6082 & 4.04 & -0.03 &   6.4 &    &     6381 &     4.34 &      P12 \\
 KOI-2678 &   6779260 & 5397 & 4.65 &  0.03 &   6.5 &    &     5371 &     4.00 &      P12 \\
 KOI-2681 &   6878240 & 5368 & 4.51 & -0.17 & < 2.0 &    &     5292 &     4.62 &      P12 \\
 KOI-2686 &   7826659 & 4743 & 4.54 & -0.04 & < 2.0 &    &     4724 &     4.64 &      P12 \\
 KOI-2687 &   7202957 & 5828 & 4.61 &  0.05 &   2.5 &    &     5804 &     3.91 &      P12 \\
 KOI-2690 &   5369827 & 5509 & 4.66 &  0.10 &   2.5 &    &     5601 &     4.33 &      P12 \\
 KOI-2694 &   9475552 & 4808 & 4.53 &  0.18 &   2.2 &    &     4706 &     4.64 &      P12 \\
 KOI-2698 &   5128673 & 5970 & 4.31 &  0.08 & < 2.0 &    &     5820 &     4.54 &      P12 \\
 KOI-2706 &   9697131 & 6277 & 4.08 &  0.06 &  10.6 &    &     6492 &     4.15 &      P12 \\
 KOI-2707 &   5480640 & 5613 & 4.35 & -0.12 & < 2.0 &    &     5610 &     4.58 &      P12 \\
 KOI-2711 &   5272233 & 5959 & 4.53 &  0.04 &   3.5 &    &     6062 &     4.35 &      P12 \\
 KOI-2712 &  11098013 & 6277 & 4.08 &  0.20 &  13.2 &    &     6457 &     4.26 &      P12 \\
 KOI-2714 &  12206313 & 5996 & 4.05 & -0.07 &   5.4 &    &     6363 &     4.19 &      P12 \\
 KOI-2717 &   9467404 & 6026 & 4.20 & -0.06 &   4.1 &    &     6430 &     4.25 &      P12 \\
 KOI-2720 &   8176564 & 6017 & 4.19 & -0.16 &   2.6 &    &     6108 &     4.41 &      P12 \\
 KOI-2722 &   7673192 & 6152 & 4.32 & -0.12 &   6.2 &    &     6536 &     4.34 &      P12 \\
 KOI-2729 &  12008872 & 5590 & 3.95 & -0.38 & < 2.0 &    &     6145 &     4.35 &      P12 \\
 KOI-2730 &   8415200 & 5599 & 3.92 & -0.05 & < 2.0 &    &     5928 &     4.51 &      P12 \\
 KOI-2732 &   9886361 & 6017 & 4.00 & -0.01 &   4.2 &    &     6310 &     4.44 &      P12 \\
 KOI-2733 &   5953297 & 4858 & 4.65 & -0.00 &   3.4 &    &     4809 &     4.62 &      P12 \\
 KOI-2737 &   6614629 & 5603 & 4.00 &  0.31 & < 2.0 &    &     5629 &     4.36 &      P12 \\
 KOI-2740 &   3336765 & 6017 & 4.27 & -0.37 &   6.5 &    &     6178 &     4.39 &      P12 \\
 KOI-2741 &   5513893 & 5805 & 4.35 & -0.01 & < 2.0 &    &     5968 &     4.52 &      P12 \\
 KOI-2743 &   8095441 & 5534 & 4.36 & -0.07 & < 2.0 &    &     5642 &     4.56 &      P12 \\
 KOI-2748 &   9962455 & 5496 & 3.81 & -0.15 & < 2.0 &    &     5689 &     4.57 &      P12 \\
 KOI-2749 &   8687088 & 6179 & 4.00 & -0.06 &   9.4 &    &     5780 &     4.44 &      Sol \\
 KOI-2750 &   3663173 & 5978 & 3.85 & -0.17 &   7.9 &    &     6116 &     4.74 &      KIC \\
 KOI-2752 &   5717567 & 6042 & 4.17 &  0.08 &   7.2 &    &     6107 &     4.36 &      P12 \\
 KOI-2753 &   6265792 & 5827 & 4.24 &  0.18 &   2.0 &    &     5983 &     4.36 &      P12 \\
 KOI-2754 &  10905911 & 5913 & 4.43 & -0.16 & < 2.0 &    &     5780 &     4.44 &      Sol \\
 KOI-2755 &   3545135 & 5756 & 4.45 & -0.23 & < 2.0 &    &     5996 &     4.46 &      P12 \\
 KOI-2756 &   6964929 & 5911 & 4.38 &  0.05 &   2.4 &    &     5928 &     4.53 &      P12 \\
 KOI-2758 &   8703129 & 5210 & 3.74 &  0.29 &   2.7 &    &     5137 &     3.14 &      P12 \\
 KOI-2763 &   3834322 & 4799 & 4.61 & -0.03 & < 2.0 &    &     4739 &     4.64 &      P12 \\
 KOI-2765 &  11188249 & 6184 & 4.03 &  0.02 &   2.5 &    &     5780 &     4.44 &      Sol \\
 KOI-2768 &   9008737 & 5337 & 4.51 & -0.09 & < 2.0 &    &     5599 &     4.58 &      P12 \\
 KOI-2769 &   9692128 & 5771 & 3.98 & -0.11 & < 2.0 &    &     6011 &     4.33 &      P12 \\
 KOI-2771 &  11456382 & 6210 & 4.40 & -0.09 &   3.8 &    &     5780 &     4.44 &      Sol \\
 KOI-2781 &   8190354 & 5722 & 4.09 & -0.56 & < 2.0 &    &     5686 &     4.43 &      P12 \\
 KOI-2785 &  10001368 & 5851 & 4.34 & -0.05 & < 2.0 &    &     5986 &     4.38 &      KIC \\
 KOI-2786 &   9466429 & 6277 & 4.14 & -0.25 &   7.1 &    &     6773 &     4.23 &      P12 \\
 KOI-2790 &   5652893 & 5106 & 4.18 & -0.26 & < 2.0 &    &     5188 &     4.62 &      P12 \\
 KOI-2792 &  11127479 & 5986 & 4.19 &  0.18 &   2.9 &    &     6000 &     4.44 &      P12 \\
 KOI-2796 &  11246161 & 5719 & 4.39 & -0.06 & < 2.0 &    &     6086 &     4.49 &      P12 \\
 KOI-2801 &   5905822 & 6017 & 4.11 & -0.03 &   3.4 &    &     6097 &     3.89 &      P12 \\
 KOI-2803 &   9898447 & 5636 & 4.42 &  0.14 & < 2.0 &    &     5632 &     4.57 &      P12 \\
 KOI-2805 &  11135308 & 5828 & 4.22 & -0.34 & < 2.0 &    &     6336 &     4.32 &      P12 \\
 KOI-2807 &   2985587 & 6302 & 4.14 &  0.08 &  13.7 &    &     6286 &     4.28 &      P12 \\
 KOI-2815 &   9665922 & 5840 & 4.18 & -0.13 & < 2.0 &    &     5824 &     4.54 &      P12 \\
 KOI-2829 &   6197215 & 5893 & 4.13 & -0.05 &   3.0 &    &     6193 &     4.26 &      P12 \\
 KOI-2831 &   9692557 & 5755 & 3.99 & -0.07 &   3.6 &    &     5890 &     4.53 &      P12 \\
 KOI-2832 &   9995402 & 5027 & 4.43 &  0.07 & < 2.0 &    &     5124 &     4.54 &      P12 \\
 KOI-2833 &   9109857 & 6132 & 4.29 & -0.32 &   4.5 &    &     6067 &     3.97 &      P12 \\
 KOI-2838 &   6607357 & 5688 & 4.01 &  0.10 & < 2.0 &    &     5789 &     4.51 &      P12 \\
 KOI-2840 &   6467363 & 5662 & 3.90 & -0.05 & < 2.0 &    &     5731 &     4.47 &      P12 \\
 KOI-2841 &   8758204 & 5133 & 4.17 & -0.36 & < 2.0 &    &     5361 &     4.61 &      P12 \\
 KOI-2848 &   7749773 & 5746 & 4.24 &  0.31 & < 2.0 &    &     5770 &     3.97 &      P12 \\
 KOI-2857 &   6345732 & 6160 & 4.10 &  0.18 &   6.2 &    &     6231 &     4.32 &      P12 \\
 KOI-2859 &  10397751 & 5252 & 4.35 & -0.10 & < 2.0 &    &     5464 &     4.47 &      P12 \\
 KOI-2863 &   3241557 & 5652 & 3.96 & -0.34 & < 2.0 &    &     6053 &     4.50 &      P12 \\
 KOI-2864 &   3957082 & 5756 & 4.31 & -0.23 & < 2.0 &    &     6084 &     4.39 &      P12 \\
 KOI-2866 &   4138951 & 6298 & 4.29 &  0.06 &   5.1 &    &     6365 &     4.43 &      P12 \\
 KOI-2874 &   9149789 & 5271 & 4.31 & -0.10 & < 2.0 &    &     5485 &     4.59 &      P12 \\
 KOI-2875 &  12170648 & 5025 & 4.61 & -0.10 & < 2.0 &    &     5160 &     4.55 &      P12 \\
 KOI-2879 &   7051984 & 5510 & 4.55 & -0.04 & < 2.0 &    &     5603 &     3.86 &      P12 \\
 KOI-2884 &   9652649 & 5728 & 4.02 & -0.07 & < 2.0 &    &     5642 &     4.51 &      P12 \\
 KOI-2885 &  11100670 & 5502 & 3.70 & -0.48 & < 2.0 &    &     5322 &     4.63 &      KIC \\
 KOI-2891 &  10068024 & 6041 & 3.98 &  0.05 &   5.5 &    &     6351 &     4.42 &      P12 \\
 KOI-2896 &   2853828 & 6181 & 4.39 & -0.09 &  14.8 &    &     6331 &     4.25 &      P12 \\
 KOI-2904 &   3969687 & 6056 & 3.97 &  0.25 &   7.2 &    &     5983 &     4.51 &      P12 \\
 KOI-2906 &   6716545 & 6017 & 4.11 & -0.39 &   5.5 &    &     6326 &     4.25 &      P12 \\
 KOI-2913 &   9693006 & 5756 & 4.30 &  0.30 & < 2.0 &    &     5743 &     4.56 &      P12 \\
 KOI-2915 &   5613821 & 5574 & 4.27 & -0.04 & < 2.0 &    &     5780 &     4.44 &      Sol \\
 KOI-2916 &   7269881 & 5033 & 4.56 & -0.02 & < 2.0 &    &     5084 &     4.58 &      P12 \\
 KOI-2925 &   6974658 & 5433 & 4.45 &  0.14 & < 2.0 &    &     5520 &     4.37 &      P12 \\
 KOI-2931 &   8611257 & 4975 & 4.53 & -0.22 & < 2.0 &    &     5084 &     4.64 &      P12 \\
 KOI-2943 &   9838468 & 5756 & 4.07 &  0.29 & < 2.0 &    &     5880 &     4.53 &      P12 \\
 KOI-2949 &   6026737 & 5913 & 4.17 &  0.02 & < 2.0 &    &     6173 &     4.00 &      P12 \\
 KOI-2951 &   4991208 & 5652 & 4.38 & -0.24 & < 2.0 &    &     5789 &     4.55 &      P12 \\
 KOI-2956 &   8801316 & 6398 & 4.08 & -0.03 &   9.6 &    &     6719 &     4.18 &      P12 \\
 KOI-2960 &  10876237 & 6007 & 4.30 &  0.06 & < 2.0 &    &     6228 &     4.46 &      P12 \\
 KOI-2961 &  10471515 & 6116 & 4.29 &  0.10 &   4.6 &    &     6460 &     3.99 &      P12 \\
 KOI-2964 &  10098844 & 6046 & 4.06 & -0.45 &   8.0 &    &     5906 &     4.45 &      P12 \\
 KOI-2968 &   8873090 & 6237 & 4.08 & -0.18 &   6.9 &    &     5780 &     4.44 &      Sol \\
 KOI-2969 &   8560804 & 6002 & 4.04 &  0.15 &   4.5 &    &     6127 &     4.44 &      P12 \\
 KOI-2970 &   5450893 & 6156 & 4.27 & -0.13 &   4.8 &    &     6475 &     4.27 &      P12 \\
 KOI-2971 &   4770174 & 6171 & 4.05 &  0.08 &  14.8 &    &     6231 &     4.43 &      P12 \\
 KOI-2974 &   3336283 & 6426 & 4.05 &  0.02 &  13.0 &    &     6480 &     4.40 &      P12 \\
 KOI-2977 &  11090556 & 5955 & 4.19 & -0.11 & < 2.0 &    &     6265 &     4.44 &      P12 \\
 KOI-2979 &   2720514 & 5985 & 4.26 & -0.26 & < 2.0 &    &     6206 &     4.38 &      P12 \\
 KOI-2984 &   7918652 & 6077 & 4.05 &  0.03 &   6.1 &    &     6032 &     4.25 &      P12 \\
 KOI-3008 &   9070666 & 6009 & 4.08 & -0.12 &   5.0 &    &     6052 &     4.29 &      KIC \\
 KOI-3009 &  12405333 & 5111 & 4.61 &  0.09 & < 2.0 &    &     5191 &     4.53 &      P12 \\
 KOI-3012 &   7109851 & 5471 & 3.70 & -0.60 & < 2.0 &    &     5945 &     3.91 &      P12 \\
 KOI-3015 &  11403530 & 5756 & 4.09 & -0.09 & < 2.0 &    &     6093 &     4.46 &      P12 \\
 KOI-3017 &  12072872 & 5493 & 4.21 & -0.24 & < 2.0 &    &     5933 &     4.38 &      P12 \\
 KOI-3021 &   3348285 & 5924 & 4.51 &  0.17 & < 2.0 &    &     6234 &     4.46 &      P12 \\
 KOI-3023 &   7732285 & 6239 & 4.26 & -0.18 &   6.4 &    &     5780 &     4.44 &      Sol \\
 KOI-3032 &  10585738 & 5173 & 4.42 &  0.29 & < 2.0 &    &     5173 &     4.57 &      P12 \\
 KOI-3039 &   5445681 & 5754 & 4.11 & -0.32 & < 2.0 &    &     5963 &     4.41 &      P12 \\
 KOI-3046 &   8161830 & 5666 & 4.17 &  0.25 & < 2.0 &    &     5635 &     4.57 &      P12 \\
 KOI-3052 &   8827575 & 5421 & 4.57 & -0.19 &   2.3 &    &     5453 &     4.42 &      P12 \\
 KOI-3060 &  11019987 & 6221 & 4.07 & -0.09 &   5.8 &    &     6529 &     4.37 &      P12 \\
 KOI-3065 &   5040077 & 5794 & 4.65 & -0.04 & < 2.0 &    &     5589 &     4.51 &      KIC \\
 KOI-3075 &   3328080 & 5346 & 4.10 & -0.52 & < 2.0 &    &     5780 &     4.44 &      Sol \\
 KOI-3083 &   7106173 & 5846 & 4.32 &  0.29 & < 2.0 &    &     5923 &     4.53 &      P12 \\
 KOI-3086 &  10749059 & 5193 & 4.24 & -0.35 & < 2.0 &    &     5278 &     4.53 &      KIC \\
 KOI-3087 &   9119568 & 5333 & 4.59 &  0.26 & < 2.0 &    &     5177 &     4.53 &      P12 \\
 KOI-3093 &   5096590 & 5881 & 4.43 &  0.00 & < 2.0 &    &     5899 &     4.53 &      P12 \\
 KOI-3096 &   7455981 & 5523 & 3.81 & -0.07 & < 2.0 &    &     5642 &     4.45 &      P12 \\
 KOI-3097 &   7582689 & 5943 & 4.06 & -0.08 &   4.6 &    &     6305 &     4.01 &      P12 \\
 KOI-3100 &   7107561 & 5967 & 4.07 &  0.25 &   2.2 &    &     6094 &     4.49 &      P12 \\
 KOI-3103 &  11237332 & 5904 & 4.26 &  0.25 &   3.0 &    &     5780 &     4.44 &      Sol \\
 KOI-3109 &  11572193 & 6245 & 4.02 &  0.03 &  17.2 &    &     5780 &     4.44 &      Sol \\
 KOI-3111 &   8581240 & 5968 & 4.39 & -0.10 & < 2.0 &    &     6033 &     3.92 &      P12 \\
 KOI-3114 &   9288237 & 6141 & 3.97 &  0.12 &   8.4 &    &     6197 &     4.45 &      P12 \\
 KOI-3117 &   6523351 & 5527 & 4.43 &  0.05 & < 2.0 &    &     5690 &     4.16 &      P12 \\
 KOI-3122 &  12416661 & 6143 & 3.96 &  0.16 &   9.9 &    &     6354 &     4.15 &      P12 \\
 KOI-3125 &   8751796 & 6258 & 4.25 & -0.20 &   9.3 &    &     6641 &     4.33 &      P12 \\
 KOI-3128 &   7609674 & 6039 & 3.94 & -0.19 &   4.8 &    &     5780 &     4.44 &      Sol \\
 KOI-3130 &  10252275 & 4889 & 4.44 & -0.55 & < 2.0 &    &     5141 &     4.54 &      P12 \\
 KOI-3132 &   9541295 & 6230 & 4.02 &  0.41 &  11.8 &    &     5995 &     4.37 &      P12 \\
 KOI-3146 &  10908248 & 5728 & 4.16 &  0.21 & < 2.0 &    &     5902 &     4.35 &      P12 \\
 KOI-3158 &   6278762 & 4990 & 4.13 & -0.50 & < 2.0 &    &     5780 &     4.44 &      Sol \\
 KOI-3165 &   9579208 & 6100 & 3.99 & -0.33 &   7.9 &    &     6424 &     4.16 &      P12 \\
 KOI-3167 &  12255382 & 5579 & 4.63 & -0.02 &   2.6 &    &     5549 &     3.80 &      P12 \\
 KOI-3168 &   4450844 & 5799 & 4.16 & -0.23 & < 2.0 &    &     5968 &     4.19 &      P12 \\
 KOI-3172 &   3337061 & 6017 & 3.97 & -0.11 &   5.9 &    &     5780 &     4.44 &      Sol \\
 KOI-3179 &   6153407 & 5742 & 4.61 &  0.04 & < 2.0 &    &     5780 &     4.44 &      Sol \\
 KOI-3180 &   3936658 & 6021 & 3.86 &  0.01 &   4.2 &    &     6250 &     3.91 &      P12 \\
 KOI-3184 &   4735826 & 5880 & 4.17 &  0.22 &   3.4 &    &     5780 &     4.44 &      Sol \\
 KOI-3190 &   5985713 & 5976 & 4.25 & -0.28 & < 2.0 &    &     5780 &     4.44 &      Sol \\
 KOI-3193 &   7430876 & 4975 & 3.17 &  0.03 &   2.2 &    &     5780 &     4.44 &      Sol \\
 KOI-3194 &  12004971 & 6294 & 4.06 &  0.12 &   6.5 &    &     6499 &     4.30 &      P12 \\
 KOI-3195 &  10118942 & 5966 & 3.93 & -0.45 &   3.1 &    &     6359 &     4.14 &      P12 \\
 KOI-3196 &   9002538 & 6092 & 4.21 & -0.06 &   2.7 &    &     6420 &     4.22 &      P12 \\
 KOI-3197 &   8443527 & 6176 & 4.40 & -0.17 &   7.0 &    &     6345 &     4.10 &      P12 \\
 KOI-3201 &   2305819 & 5709 & 4.45 & -0.54 & < 2.0 &    &     6146 &     4.13 &      P12 \\
 KOI-3202 &   4262040 & 5280 & 3.75 & -0.02 & < 2.0 &    &     5337 &     3.98 &      P12 \\
 KOI-3208 &  10155029 & 5874 & 4.48 & -0.20 & < 2.0 &    &     5780 &     4.44 &      Sol \\
 KOI-3214 &   7983117 & 5943 & 4.10 & -0.14 &   4.4 &    &     6019 &     3.62 &      P12 \\
 KOI-3215 &   3342952 & 5524 & 3.39 & -0.08 & < 2.0 &    &     5663 &     4.45 &      P12 \\
 KOI-3218 &  10191036 & 6002 & 4.42 & -0.01 &   3.1 &    &     6239 &     4.34 &      P12 \\
 KOI-3220 &  11189311 & 6300 & 4.11 &  0.04 &  12.7 &    &     5780 &     4.44 &      Sol \\
 KOI-3224 &  10384298 & 5404 & 4.59 &  0.04 & < 2.0 &    &     5429 &     4.60 &      P12 \\
 KOI-3225 &   3109550 & 5416 & 4.56 &  0.14 & < 2.0 &    &     5449 &     4.03 &      P12 \\
 KOI-3227 &   8975368 & 5950 & 4.32 & -0.02 & < 2.0 &    &     6051 &     4.10 &      P12 \\
 KOI-3232 &   9569711 & 5813 & 4.61 &  0.03 &   3.0 &    &     5830 &     4.13 &      P12 \\
 KOI-3233 &   2142501 & 5756 & 4.47 & -0.03 & < 2.0 &    &     5780 &     4.44 &      Sol \\
 KOI-3234 &  10057494 & 6376 & 4.42 & -0.15 &  11.7 &    &     6393 &     4.35 &      P12 \\
 KOI-3236 &   7902003 & 6258 & 4.13 & -0.01 &  13.1 &    &     6437 &     4.37 &      P12 \\
 KOI-3237 &   6587796 & 5871 & 4.59 &  0.18 &   4.4 &    &     5814 &     4.55 &      P12 \\
 KOI-3239 &   5305240 & 5664 & 4.63 &  0.02 &   4.9 &    &     5688 &     4.12 &      P12 \\
 KOI-3240 &   6206559 & 6017 & 3.88 &  0.20 &   4.9 &    &     5780 &     4.44 &      Sol \\
 KOI-3244 &   6850665 & 4974 & 3.02 & -0.08 &   3.3 &    &     5047 &     3.73 &      P12 \\
 KOI-3245 &   8073705 & 6091 & 4.25 & -0.18 & < 2.0 &    &     6223 &     4.34 &      P12 \\
 KOI-3246 &   9885417 & 4832 & 4.61 &  0.11 &   2.4 &    &     4725 &     4.64 &      P12 \\
 KOI-3248 &  10917433 & 5719 & 4.29 & -0.07 & < 2.0 &    &     6005 &     4.16 &      P12 \\
 KOI-3249 &   9083564 & 6028 & 4.27 & -0.00 &   3.4 &    &     5954 &     4.30 &      KIC \\
 KOI-3251 &   8413968 & 5939 & 4.21 &  0.03 &   2.9 &    &     6177 &     4.29 &      P12 \\
 KOI-3254 &   9899141 & 5573 & 4.25 &  0.26 & < 2.0 &    &     5570 &     4.33 &      P12 \\
 KOI-3277 &   3120904 & 6007 & 3.98 & -0.07 &   7.0 &    &     5972 &     4.52 &      P12 \\
 KOI-3278 &   3342467 & 5489 & 4.62 &  0.16 &   3.4 &    &     5414 &     4.61 &      P12 \\
 KOI-3287 &   6584273 & 5896 & 4.24 & -0.18 & < 2.0 &    &     5979 &     4.51 &      P12 \\
 KOI-3288 &   5768816 & 5462 & 4.65 &  0.03 & < 2.0 &    &     5613 &     4.41 &      P12 \\
 KOI-3301 &   8301878 & 5756 & 4.02 &  0.23 &   2.1 &    &     5613 &     4.47 &      P12 \\
 KOI-3308 &   3632089 & 5861 & 4.08 & -0.04 &   2.7 &    &     5683 &     4.37 &      P12 \\
 KOI-3310 &  12253769 & 5416 & 4.38 &  0.18 & < 2.0 &    &     5544 &     4.53 &      P12 \\
 KOI-3315 &   8554701 & 5594 & 4.08 & -0.50 & < 2.0 &    &     6106 &     4.49 &      P12 \\
 KOI-3338 &   8263752 & 6096 & 4.25 & -0.29 & < 2.0 &    &     6571 &     4.34 &      P12 \\
 KOI-3340 &   3529290 & 6092 & 4.29 & -0.18 &   6.1 &    &     6208 &     4.45 &      P12 \\
 KOI-3346 &  11241912 & 5930 & 4.27 & -0.07 & < 2.0 &    &     6179 &     4.37 &      P12 \\
 KOI-3358 &   4263529 & 5438 & 4.52 & -0.12 &   2.2 &    &     5520 &     4.53 &      P12 \\
 KOI-3363 &  11651712 & 5670 & 4.02 & -0.11 & < 2.0 &    &     5996 &     4.51 &      P12 \\
 KOI-3371 &  11125797 & 5544 & 4.65 &  0.01 & < 2.0 &    &     5444 &     4.59 &      P12 \\
 KOI-3378 &   4376629 & 5496 & 4.02 & -0.51 & < 2.0 &    &     5946 &     4.52 &      P12 \\
 KOI-3382 &   9991621 & 5371 & 4.32 &  0.13 & < 2.0 &    &     5456 &     4.42 &      P12 \\
 KOI-3384 &   8644365 & 6017 & 4.24 &  0.03 &   2.7 &    &     5984 &     4.24 &      P12 \\
 KOI-3403 &  11754430 & 5765 & 4.04 &  0.06 &   3.0 &    &     6028 &     4.31 &      P12 \\
 KOI-3419 &  11519134 & 6314 & 3.61 & -0.62 &   4.1 &    &     6388 &     4.20 &      P12 \\
 KOI-3421 &   5004909 & 6277 & 4.12 &  0.01 &   7.6 &    &     6487 &     4.40 &      P12 \\
 KOI-3422 &   5898983 & 5888 & 4.60 &  0.10 &   4.5 &    &     5944 &     4.44 &      P12 \\
 KOI-3425 &   9117416 & 6055 & 3.96 & -0.07 &   6.1 &    &     5780 &     4.44 &      Sol \\
 KOI-3436 &   6265665 & 5071 & 4.67 &  0.18 &   2.4 &    &     5018 &     3.82 &      P12 \\
 KOI-3438 &   6599975 & 6017 & 4.38 & -0.25 &   2.8 &    &     6394 &     4.38 &      P12 \\
 KOI-3451 &  10793576 & 6017 & 4.38 & -0.01 &   2.2 &    &     6172 &     4.38 &      KIC \\
 KOI-3456 &   6364582 & 5604 & 4.36 & -0.34 &   7.9 &    &     6012 &     4.37 &      P12 \\
 KOI-3465 &   9763612 & 5359 & 4.59 &  0.03 & < 2.0 &    &     5430 &     4.02 &      P12 \\
 KOI-3473 &   8905246 & 5155 & 4.66 & -0.01 &   4.7 &    &     5156 &     3.79 &      P12 \\
 KOI-3474 &   5213230 & 5907 & 4.24 & -0.23 &   3.8 &    &     5805 &     4.55 &      P12 \\
 KOI-3497 &   8424002 & 4825 & 4.63 &  0.08 &   4.0 &    &     5780 &     4.44 &      Sol \\
 KOI-3500 &   6058816 & 6017 & 3.96 &  0.15 &   6.4 &    &     6093 &     4.47 &      P12 \\
 KOI-3503 &   6368175 & 6017 & 4.33 & -0.60 & < 2.0 &    &     6398 &     4.42 &      P12 \\
 KOI-3541 &   8868364 & 6073 & 4.09 & -0.37 &   6.4 &    &     5780 &     4.44 &      Sol \\
 KOI-3608 &  10259301 & 5895 & 4.37 & -0.11 & < 2.0 &    &     6111 &     4.45 &      P12 \\
 KOI-3641 &   3534118 & 6170 & 4.21 & -0.17 & < 2.0 &    &     5986 &     4.51 &      P12 \\
 KOI-3663 &  12735740 & 5700 & 4.38 & -0.07 & < 2.0 &    &     5983 &     4.34 &      P12 \\
 KOI-3678 &   4150804 & 5496 & 4.48 &  0.14 & < 2.0 &    &     5780 &     4.44 &      Sol \\
 KOI-3680 &   9025971 & 5804 & 4.40 &  0.11 & < 2.0 &    &     5921 &     4.53 &      P12 \\
 KOI-3681 &   2581316 & 6213 & 4.25 &  0.10 &   7.9 &    &     5780 &     4.44 &      Sol \\
 KOI-3683 &  10795103 & 6301 & 4.12 & -0.09 &  10.6 &    &     6515 &     4.28 &      P12 \\
 KOI-3689 &   7017372 & 5986 & 4.16 & -0.04 &   3.4 &    &     6206 &     4.24 &      KIC \\
 KOI-3770 &   5008245 & 6087 & 4.06 & -0.12 &   6.1 &    &     6118 &     4.39 &      KIC \\
 KOI-3780 &   6775985 & 6201 & 3.95 & -0.37 &   8.5 &    &     6540 &     4.24 &      KIC \\
 KOI-3787 &   7813039 & 5737 & 4.58 &  0.11 & < 2.0 &    &     5973 &     4.36 &      P12 \\
 KOI-3791 &   5437945 & 6061 & 4.00 & -0.07 &   4.6 &    &     6374 &     4.18 &      P12 \\
 KOI-3801 &   8827930 & 5671 & 4.16 &  0.14 &   2.5 &    &     5681 &     4.57 &      P12 \\
 KOI-3811 &   4638237 & 5795 & 4.44 & -0.24 &   3.6 &    &     5650 &     4.46 &      P12 \\
 KOI-3823 &   4820550 & 5631 & 4.47 &  0.06 & < 2.0 &    &     5796 &     4.55 &      P12 \\
 KOI-3835 &   2581554 & 5023 & 4.70 &  0.00 &   4.4 &    &     5016 &     3.82 &      P12 \\
 KOI-3853 &   2697935 & 4888 & 3.37 & -0.16 &   2.6 &    &     4883 &     3.27 &      KIC \\
 KOI-3864 &   4164922 & 5057 & 4.68 &  0.05 &   3.9 &    &     5026 &     3.83 &      P12 \\
 KOI-3867 &   9353742 & 5552 & 4.36 &  0.07 & < 2.0 &    &     5774 &     4.55 &      P12 \\
 KOI-3871 &   9752982 & 5206 & 4.62 &  0.04 & < 2.0 &    &     5154 &     3.79 &      P12 \\
 KOI-3876 &   3440118 & 5721 & 4.72 &  0.07 &   9.8 &    &     5853 &     4.24 &      P12 \\
 KOI-3880 &   4147444 & 6251 & 4.37 &  0.02 &  14.3 &    &     5780 &     4.44 &      Sol \\
 KOI-3886 &   8848288 & 4726 & 2.99 &  0.15 &   5.1 &    &     4842 &     2.54 &      P12 \\
 KOI-3889 &  10733174 & 5756 & 4.24 &  0.16 & < 2.0 &    &     5857 &     4.54 &      P12 \\
 KOI-3890 &   8564976 & 4788 & 2.92 & -0.19 &   2.2 &    &     5020 &     3.17 &      P12 \\
 KOI-3891 &   8765560 & 5121 & 3.64 & -0.12 & < 2.0 &    &     5304 &     3.60 &      P12 \\
 KOI-3892 &  11760860 & 5693 & 4.39 &  0.27 & < 2.0 &    &     5763 &     4.55 &      P12 \\
 KOI-3907 &   7137213 & 6400 & 4.31 & -0.21 &  18.5 &    &     6516 &     4.09 &      P12 \\
 KOI-3908 &  10363115 & 5756 & 4.01 & -0.00 &   3.5 &    &     5887 &     3.48 &      P12 \\
 KOI-3913 &  10281221 & 6017 & 4.32 &  0.16 & < 2.0 &    &     6268 &     4.45 &      P12 \\
 KOI-3925 &  10788461 & 5390 & 4.63 &  0.03 & < 2.0 &    &     5457 &     4.21 &      KIC \\
 KOI-3928 &   4242692 & 6189 & 4.25 & -0.10 &   6.3 &    &     6543 &     4.09 &      P12 \\
 KOI-3936 &   4947556 & 5085 & 4.68 &  0.12 &   5.7 &    &     4982 &     4.59 &      P12 \\
 KOI-3943 &   7679812 & 6210 & 4.20 & -0.10 &   7.5 &    &     6484 &     4.19 &      P12 \\
 KOI-3946 &   8636434 & 6272 & 4.15 & -0.32 &   7.0 &    &     6371 &     4.43 &      P12 \\
 KOI-3980 &   6750902 & 5756 & 4.35 &  0.10 &   2.0 &    &     5904 &     4.40 &      P12 \\
 KOI-3991 &  10352333 & 5672 & 4.61 & -0.05 &   6.2 &    &     5702 &     4.35 &      P12 \\
 KOI-4002 &   5773121 & 5218 & 4.58 &  0.14 & < 2.0 &    &     5224 &     4.51 &      P12 \\
 KOI-4004 &   4814502 & 5781 & 4.72 & -0.05 &   6.6 &    &     5835 &     3.85 &      P12 \\
 KOI-4005 &   8142787 & 5474 & 4.36 &  0.02 & < 2.0 &    &     5605 &     4.58 &      P12 \\
 KOI-4011 &  11969988 & 5972 & 4.24 &  0.16 &   3.0 &    &     6181 &     4.36 &      P12 \\
 KOI-4014 &   9009953 & 5995 & 4.37 &  0.04 &   2.9 &    &     6221 &     4.46 &      P12 \\
 KOI-4018 &   4929299 & 5465 & 4.44 & -0.07 & < 2.0 &    &     5531 &     4.33 &      KIC \\
 KOI-4022 &   7733731 & 6017 & 4.06 & -0.13 &   6.6 &    &     6138 &     4.34 &      P12 \\
 KOI-4024 &  10714072 & 5298 & 4.56 & -0.05 &   3.0 &    &     5337 &     3.98 &      P12 \\
 KOI-4032 &   7100673 & 5584 & 4.18 &  0.04 & < 2.0 &    &     5744 &     4.23 &      P12 \\
 KOI-4036 &  11415243 & 4880 & 4.58 & -0.00 & < 2.0 &    &     4859 &     4.61 &      P12 \\
 KOI-4037 &   8264402 & 6204 & 4.21 & -0.08 &   7.3 &    &     6537 &     4.24 &      P12 \\
 KOI-4053 &   1718958 & 6079 & 4.55 & -0.12 &   3.8 &    &     6176 &     4.42 &      P12 \\
 KOI-4060 &   9086154 & 5761 & 4.11 &  0.10 &   2.3 &    &     6006 &     4.51 &      P12 \\
 KOI-4062 &  11858979 & 6017 & 4.13 & -0.05 &   3.3 &    &     5990 &     4.32 &      KIC \\
 KOI-4066 &   8686373 & 6277 & 4.20 &  0.03 &  12.6 &    &     5780 &     4.44 &      Sol \\
 KOI-4067 &   5530112 & 6017 & 4.33 &  0.05 &   3.4 &    &     6221 &     4.35 &      KIC \\
 KOI-4070 &  10186945 & 4931 & 4.52 &  0.02 & < 2.0 &    &     4988 &     4.58 &      P12 \\
 KOI-4072 &   6755944 & 5863 & 4.25 &  0.08 & < 2.0 &    &     6113 &     4.40 &      P12 \\
 KOI-4098 &   8222627 & 5038 & 4.64 & -0.08 & < 2.0 &    &     4970 &     3.67 &      P12 \\
 KOI-4103 &   3747817 & 5340 & 4.62 & -0.08 & < 2.0 &    &     5294 &     4.62 &      P12 \\
 KOI-4109 &   7907808 & 4981 & 4.50 &  0.21 & < 2.0 &    &     4927 &     3.71 &      P12 \\
 KOI-4123 &   6140059 & 6167 & 3.93 &  0.06 &   3.2 &    &     6209 &     4.26 &      P12 \\
 KOI-4129 &  11970988 & 5116 & 4.55 &  0.14 & < 2.0 &    &     5161 &     4.53 &      P12 \\
 KOI-4136 &   7256914 & 5741 & 4.07 &  0.12 &   2.2 &    &     5761 &     4.55 &      P12 \\
 KOI-4144 &   3112129 & 6017 & 4.39 & -0.20 & < 2.0 &    &     6057 &     4.47 &      P12 \\
 KOI-4146 &  10000941 & 5081 & 4.66 &  0.20 &   3.2 &    &     5056 &     4.57 &      P12 \\
 KOI-4156 &   5881120 & 5788 & 4.05 &  0.22 & < 2.0 &    &     5995 &     4.51 &      P12 \\
 KOI-4157 &   4548098 & 6238 & 4.25 & -0.03 &  10.1 &    &     6567 &     4.30 &      P12 \\
 KOI-4159 &   6607644 & 5185 & 4.31 &  0.05 & < 2.0 &    &     5337 &     4.61 &      P12 \\
 KOI-4160 &   7610663 & 5800 & 4.61 &  0.23 & < 2.0 &    &     5739 &     4.40 &      P12 \\
 KOI-4184 &   6752002 & 4918 & 4.58 & -0.02 &   4.6 &    &     4936 &     4.59 &      P12 \\
 KOI-4188 &   6879171 & 5966 & 4.44 &  0.06 &   3.2 &    &     5780 &     4.44 &      Sol \\
 KOI-4190 &  12505503 & 5676 & 4.09 &  0.27 & < 2.0 &    &     5722 &     4.56 &      P12 \\
 KOI-4198 &   9072639 & 6032 & 3.96 & -0.48 &   5.5 &    &     5780 &     4.44 &      Sol \\
 KOI-4199 &   5340878 & 5103 & 4.45 & -0.23 & < 2.0 &    &     5211 &     4.64 &      P12 \\
 KOI-4204 &  10593535 & 5880 & 4.23 &  0.11 &   2.2 &    &     6165 &     4.48 &      P12 \\
 KOI-4212 &   1724719 & 6179 & 4.27 &  0.08 &   6.1 &    &     6176 &     4.39 &      P12 \\
 KOI-4215 &   9366617 & 5396 & 3.64 & -0.35 & < 2.0 &    &     5469 &     3.81 &      P12 \\
 KOI-4222 &   9183378 & 5651 & 4.57 & -0.06 &   2.0 &    &     5715 &     4.07 &      P12 \\
 KOI-4226 &   9491832 & 5874 & 3.96 &  0.34 &   4.2 &    &     5641 &     4.05 &      P12 \\
 KOI-4230 &   9872831 & 5854 & 4.13 & -0.45 & < 2.0 &    &     5780 &     4.44 &      Sol \\
 KOI-4235 &  10794974 & 6277 & 4.16 & -0.03 &  13.5 &    &     6627 &     4.33 &      P12 \\
 KOI-4245 &  12737015 & 6017 & 3.99 &  0.17 &   5.0 &    &     6165 &     4.39 &      P12 \\
 KOI-4246 &   5177859 & 5706 & 4.68 &  0.25 &   5.9 &    &     5752 &     4.28 &      P12 \\
 KOI-4251 &   8741470 & 5584 & 4.60 &  0.02 & < 2.0 &    &     5713 &     4.31 &      P12 \\
 KOI-4257 &   7901016 & 5496 & 3.75 & -0.04 & < 2.0 &    &     5733 &     3.95 &      P12 \\
 KOI-4269 &   8890924 & 5011 & 3.59 &  0.04 &   2.1 &    &     5120 &     3.62 &      P12 \\
 KOI-4273 &   9716028 & 6083 & 4.07 &  0.02 &   5.3 &    &     6274 &     4.22 &      P12 \\
 KOI-4276 &   6026924 & 6203 & 3.98 &  0.07 &   8.0 &    &     5780 &     4.44 &      Sol \\
 KOI-4287 &  11081504 & 6236 & 4.19 & -0.09 &   8.3 &    &     6337 &     4.15 &      P12 \\
 KOI-4288 &   4548011 & 5953 & 4.17 &  0.04 &   2.4 &    &     6226 &     4.19 &      P12 \\
 KOI-4292 &  10063208 & 5498 & 4.09 & -0.01 & < 2.0 &    &     5780 &     4.55 &      P12 \\
 KOI-4296 &   7661893 & 5618 & 4.08 & -0.58 & < 2.0 &    &     6175 &     4.34 &      P12 \\
 KOI-4301 &   8773015 & 6115 & 4.31 & -0.32 &   4.6 &    &     6261 &     3.87 &      P12 \\
 KOI-4302 &   6290935 & 6107 & 4.13 & -0.20 &   5.2 &    &     6555 &     4.28 &      P12 \\
 KOI-4304 &  11612280 & 5836 & 4.06 & -0.01 &   2.2 &    &     6176 &     4.46 &      P12 \\
 KOI-4318 &   9286088 & 6402 & 4.27 & -0.13 &  18.2 &    &     6703 &     4.27 &      P12 \\
 KOI-4323 &   5385410 & 6269 & 4.20 & -0.16 &  10.8 &    &     6279 &     4.13 &      P12 \\
 KOI-4329 &  12456063 & 6213 & 4.18 &  0.04 &   7.7 &    &     6352 &     4.43 &      P12 \\
 KOI-4335 &  10730070 & 5691 & 4.06 & -0.40 & < 2.0 &    &     6193 &     4.40 &      P12 \\
 KOI-4343 &   8087812 & 5829 & 4.02 & -0.53 &   3.1 &    &     6014 &     4.17 &      P12 \\
 KOI-4366 &  10647452 & 5304 & 4.40 & -0.21 & < 2.0 &    &     5182 &     4.61 &      KIC \\
 KOI-4367 &   4773392 & 6277 & 4.17 & -0.12 &   7.5 &    &     6271 &     4.45 &      P12 \\
 KOI-4368 &   5471489 & 5988 & 3.94 &  0.06 &   3.5 &    &     6218 &     3.83 &      P12 \\
 KOI-4374 &  10991114 & 5397 & 4.35 & -0.00 & < 2.0 &    &     5521 &     4.59 &      P12 \\
 KOI-4382 &   6937529 & 6241 & 4.22 & -0.19 &   9.7 &    &     6478 &     4.40 &      P12 \\
 KOI-4383 &   9883606 & 5816 & 4.62 &  0.03 & < 2.0 &    &     6141 &     4.37 &      P12 \\
 KOI-4385 &   3645438 & 5119 & 4.40 &  0.02 & < 2.0 &    &     5098 &     4.63 &      KIC \\
 KOI-4399 &   8345384 & 5538 & 4.55 & -0.08 & < 2.0 &    &     5750 &     3.80 &      P12 \\
 KOI-4400 &   2831055 & 5822 & 4.41 &  0.00 & < 2.0 &    &     5957 &     4.37 &      P12 \\
 KOI-4407 &   8396660 & 6385 & 4.20 & -0.25 &   7.0 &    &     6346 &     4.08 &      P12 \\
 KOI-4409 &   5308537 & 5942 & 4.27 &  0.21 &   3.0 &    &     5896 &     4.45 &      P12 \\
 KOI-4411 &   5281113 & 6022 & 4.34 & -0.28 &   4.0 &    &     6273 &     4.45 &      P12 \\
 KOI-4421 &   9836563 & 6017 & 4.15 &  0.01 &   4.3 &    &     6196 &     4.42 &      P12 \\
 KOI-4423 &   3866536 & 6277 & 4.16 & -0.22 &   8.9 &    &     6345 &     4.42 &      P12 \\
 KOI-4426 &   8240790 & 6112 & 4.01 &  0.00 &   7.4 &    &     6279 &     4.13 &      P12 \\
 KOI-4430 &   9642018 & 5131 & 4.62 &  0.05 & < 2.0 &    &     5229 &     4.63 &      P12 \\
 KOI-4431 &   9936080 & 6152 & 4.12 & -0.28 &   9.4 &    &     5780 &     4.44 &      Sol \\
 KOI-4435 &   8278685 & 6165 & 4.07 &  0.07 &   8.7 &    &     6341 &     4.44 &      P12 \\
 KOI-4441 &   8416523 & 4915 & 4.55 &  0.05 & < 2.0 &    &     4965 &     4.61 &      P12 \\
 KOI-4443 &   5780855 & 6335 & 4.14 & -0.11 &   9.5 &    &     6673 &     4.25 &      P12 \\
 KOI-4446 &  10329196 & 5133 & 3.59 & -0.34 & < 2.0 &    &     5450 &     3.47 &      P12 \\
 KOI-4452 &   4474462 & 5756 & 4.11 & -0.37 & < 2.0 &    &     6050 &     4.17 &      P12 \\
 KOI-4457 &  12109267 & 6017 & 4.18 & -0.30 &   7.3 &    &     6399 &     4.32 &      P12 \\
 KOI-4469 &  10006641 & 4926 & 4.55 &  0.02 & < 2.0 &    &     4955 &     4.60 &      P12 \\
 KOI-4473 &   7133294 & 5928 & 3.96 & -0.03 &   5.2 &    &     5791 &     4.11 &      P12 \\
 KOI-4480 &  10467714 & 5598 & 4.37 &  0.29 & < 2.0 &    &     5637 &     4.49 &      P12 \\
 KOI-4482 &   7778427 & 6255 & 4.24 & -0.07 &   6.2 &    &     6340 &     4.25 &      P12 \\
 KOI-4505 &   8493354 & 6068 & 4.22 & -0.20 &   5.3 &    &     6579 &     4.33 &      P12 \\
 KOI-4546 &   5033823 & 5973 & 4.25 & -0.01 & < 2.0 &    &     6149 &     4.48 &      P12 \\
 KOI-4556 &  10399321 & 5496 & 3.79 & -0.16 & < 2.0 &    &     5811 &     3.83 &      P12 \\
 KOI-4557 &  10257229 & 5911 & 4.07 & -0.07 &   3.4 &    &     6202 &     4.47 &      P12 \\
 KOI-4561 &   7747457 & 6017 & 4.12 & -0.04 &   6.1 &    &     6063 &     4.27 &      KIC \\
 KOI-4567 &   8332521 & 6333 & 4.18 & -0.19 &  10.4 &    &     6153 &     4.44 &      P12 \\
 KOI-4575 &   9893468 & 6220 & 4.02 & -0.03 &   5.4 &    &     6598 &     4.12 &      P12 \\
 KOI-4580 &   8628761 & 5869 & 4.14 & -0.31 & < 2.0 &    &     6738 &     3.98 &      P12 \\
 KOI-4581 &   2572029 & 5883 & 4.30 &  0.03 & < 2.0 &    &     6076 &     4.34 &      P12 \\
 KOI-4582 &   7905106 & 5687 & 4.34 & -0.24 & < 2.0 &    &     5991 &     4.04 &      P12 \\
 KOI-4585 &   9009036 & 6092 & 4.08 & -0.23 &   9.5 &    &     6540 &     4.35 &      P12 \\
 KOI-4588 &   8806985 & 6208 & 4.08 & -0.21 &   7.0 &    &     5780 &     4.44 &      Sol \\
 KOI-4601 &  11153476 & 6175 & 4.15 &  0.15 &   7.8 &    &     6252 &     4.45 &      P12 \\
 KOI-4603 &   8430053 & 6175 & 4.16 &  0.13 &   7.8 &    &     6444 &     4.38 &      P12 \\
 KOI-4605 &  12458605 & 6017 & 3.94 & -0.03 &   3.9 &    &     6044 &     4.48 &      P12 \\
 KOI-4613 &  10220837 & 5477 & 4.41 & -0.13 & < 2.0 &    &     5708 &     4.43 &      P12 \\
 KOI-4614 &   7583650 & 6045 & 4.17 &  0.04 &   5.3 &    &     6482 &     4.22 &      P12 \\
 KOI-4617 &   9701962 & 5952 & 4.22 & -0.19 & < 2.0 &    &     6301 &     4.44 &      P12 \\
 KOI-4633 &   5954001 & 6007 & 4.11 &  0.06 &   5.3 &    &     5978 &     4.01 &      P12 \\
 KOI-4634 &   8196226 & 6042 & 4.25 &  0.07 & < 2.0 &    &     6185 &     4.40 &      P12 \\
 KOI-4637 &   9457728 & 6108 & 3.96 & -0.33 &   5.1 &    &     6387 &     4.38 &      P12 \\
 KOI-4640 &   9412623 & 6410 & 4.16 & -0.10 &  10.8 &    &     6720 &     4.32 &      P12 \\
 KOI-4647 &   9947653 & 5163 & 3.80 &  0.18 & < 2.0 &    &     5262 &     3.87 &      P12 \\
 KOI-4651 &   6717252 & 5713 & 4.66 & -0.03 & < 2.0 &    &     5595 &     4.34 &      P12 \\
 KOI-4653 &  11181260 & 6149 & 4.13 & -0.04 &   7.1 &    &     6345 &     4.43 &      P12 \\
 KOI-4657 &   6527078 & 5317 & 4.34 & -0.08 & < 2.0 &    &     5353 &     4.60 &      P12 \\
 KOI-4659 &   2857607 & 5618 & 4.38 & -0.05 & < 2.0 &    &     5870 &     4.54 &      P12 \\
 KOI-4663 &   7515336 & 5522 & 3.87 &  0.25 &   2.7 &    &     5612 &     4.18 &      P12 \\
 KOI-4665 &   7366895 & 5706 & 4.12 & -0.03 & < 2.0 &    &     5905 &     4.46 &      P12 \\
 KOI-4674 &   6839010 & 5713 & 4.32 &  0.17 & < 2.0 &    &     5757 &     4.34 &      P12 \\
 KOI-4686 &   5819801 & 5734 & 4.05 &  0.31 &   2.8 &    &     5522 &     4.08 &      P12 \\
 KOI-4693 &   8417078 & 5615 & 3.75 & -0.36 & < 2.0 &    &     6156 &     4.44 &      P12 \\
 KOI-4699 &   7891294 & 6110 & 4.23 & -0.00 &   4.5 &    &     6114 &     4.51 &      KIC \\
 KOI-4706 &  10026502 & 5916 & 4.20 & -0.37 & < 2.0 &    &     6202 &     4.40 &      P12 \\
 KOI-4715 &   6264750 & 6131 & 4.07 & -0.18 &   8.2 &    &     5780 &     4.44 &      Sol \\
 KOI-4716 &  11290515 & 6017 & 4.15 & -0.00 &   4.1 &    &     6195 &     4.34 &      P12 \\
 KOI-4717 &   4902202 & 5662 & 4.20 & -0.39 & < 2.0 &    &     5654 &     4.50 &      P12 \\
 KOI-4725 &   7778621 & 4822 & 4.42 & -0.06 & < 2.0 &    &     4911 &     3.68 &      P12 \\
 KOI-4744 &   5709906 & 5756 & 4.13 &  0.22 &   2.2 &    &     5876 &     4.53 &      P12 \\
 KOI-4745 &  11757451 & 4849 & 4.55 & -0.05 & < 2.0 &    &     4857 &     4.68 &      P12 \\
 KOI-4746 &   2711597 & 5008 & 4.63 &  0.06 &   3.9 &    &     4856 &     4.61 &      P12 \\
 KOI-4763 &   8349399 & 5744 & 4.08 &  0.13 &   2.7 &    &     5980 &     4.35 &      P12 \\
 KOI-4765 &  10615440 & 6165 & 4.20 &  0.07 &   6.2 &    &     6445 &     4.31 &      P12 \\
 KOI-4771 &  11658036 & 6277 & 4.25 & -0.15 &  10.6 &    &     6685 &     4.33 &      P12 \\
 KOI-4773 &   7906892 & 6017 & 3.94 & -0.39 &   5.7 &    &     6152 &     4.24 &      P12 \\
 KOI-4774 &   4277304 & 5222 & 4.43 & -0.04 & < 2.0 &    &     5780 &     4.44 &      Sol \\
 KOI-4775 &   8626325 & 5232 & 3.89 &  0.46 & < 2.0 &    &     5148 &     3.87 &      KIC \\
 KOI-4792 &  11618569 & 5938 & 4.47 &  0.03 & < 2.0 &    &     6208 &     4.47 &      P12 \\
 KOI-4811 &   8811490 & 5558 & 3.82 & -0.02 & < 2.0 &    &     5539 &     4.07 &      KIC \\
 KOI-4822 &   9702945 & 5804 & 4.06 & -0.08 &   2.1 &    &     6209 &     4.47 &      P12 \\
 KOI-4829 &  12401132 & 6045 & 4.18 & -0.10 &   2.9 &    &     6161 &     4.36 &      KIC \\
 KOI-4833 &  10584140 & 5756 & 4.13 & -0.02 & < 2.0 &    &     5714 &     4.19 &      KIC \\
 KOI-4834 &   8233326 & 5010 & 3.75 &  0.35 & < 2.0 &    &     5012 &     3.62 &      P12 \\
 KOI-4839 &   9110610 & 6173 & 4.18 & -0.12 & < 2.0 &    &     6222 &     3.81 &      P12 \\
 KOI-4841 &   5480884 & 4783 & 4.42 & -0.19 & < 2.0 &    &     4792 &     4.68 &      P12 \\
 KOI-4850 &   6786224 & 5516 & 4.23 & -0.00 & < 2.0 &    &     5818 &     4.54 &      P12 \\
 KOI-4864 &   7345248 & 5756 & 3.97 & -0.31 &   2.3 &    &     5919 &     4.26 &      P12 \\
 KOI-4881 &   8094120 & 6260 & 4.18 & -0.07 &   9.2 &    &     5780 &     4.44 &      Sol \\
 KOI-4887 &   4059887 & 5852 & 3.91 & -0.04 &   4.1 &    &     6077 &     4.17 &      P12 \\
 KOI-4892 &  10586744 & 5549 & 3.59 & -0.47 &   2.3 &    &     6035 &     4.31 &      P12 \\
 KOI-4907 &   5437762 & 6008 & 4.28 &  0.02 &   2.6 &    &     6357 &     4.38 &      P12 \\
 KOI-4941 &   2438406 & 5108 & 3.59 & -0.30 &   4.4 &    &     5189 &     4.35 &      KIC \\
 KOI-4961 &   3001955 & 4830 & 4.57 &  0.17 & < 2.0 &    &     4705 &     4.64 &      P12 \\
 KOI-4978 &   3428127 & 5523 & 4.57 &  0.07 & < 2.0 &    &     5337 &     4.40 &      KIC \\
 KOI-5018 &   3854101 & 5454 & 4.35 &  0.30 & < 2.0 &    &     5346 &     4.63 &      KIC \\
 KOI-5021 &   3863877 & 5725 & 4.41 & -0.00 & < 2.0 &    &     5671 &     4.57 &      P12 \\
 KOI-5039 &   4077767 & 4818 & 4.37 & -0.06 & < 2.0 &    &     4763 &     4.61 &      KIC \\
 KOI-5084 &   4760478 & 5546 & 3.87 &  0.12 & < 2.0 &    &     5430 &     4.53 &      KIC \\
 KOI-5124 &   5094412 & 5325 & 4.26 & -0.07 & < 2.0 &    &     5548 &     4.59 &      P12 \\
 KOI-5135 &   5184144 & 5161 & 4.39 & -0.05 &   2.4 &    &     5214 &     4.61 &      P12 \\
 KOI-5159 &   5397106 & 6120 & 4.27 &  0.04 &   4.0 &    &     6061 &     4.38 &      P12 \\
 KOI-5198 &   5780194 & 5377 & 4.53 & -0.02 & < 2.0 &    &     5483 &     4.59 &      P12 \\
 KOI-5216 &   5965629 & 5631 & 4.46 & -0.10 & < 2.0 &    &     5890 &     4.53 &      P12 \\
 KOI-5241 &   6139220 & 6037 & 4.07 & -0.43 &   2.8 &    &     6184 &     4.43 &      P12 \\
 KOI-5269 &   6359929 & 5351 & 4.45 & -0.22 & < 2.0 &    &     5647 &     4.49 &      P12 \\
 KOI-5423 &   7762153 & 5743 & 4.23 &  0.28 & < 2.0 &    &     5614 &     4.40 &      KIC \\
 KOI-5546 &   8571421 & 6263 & 4.48 & -0.12 &   4.8 &    &     6334 &     4.44 &      P12 \\
 KOI-5567 &   8742270 & 5542 & 4.05 &  0.05 &   2.2 &    &     5735 &     4.43 &      P12 \\
 KOI-5626 &   9147029 & 5853 & 4.12 & -0.22 & < 2.0 &    &     6341 &     4.43 &      P12 \\
 KOI-5790 &  10394802 & 4893 & 4.59 &  0.05 & < 2.0 &    &     4891 &     4.60 &      P12 \\
 KOI-5798 &  10487228 & 5033 & 4.59 & -0.04 & < 2.0 &    &     5060 &     4.66 &      P12 \\
 KOI-5837 &  10878117 & 5779 & 4.26 & -0.00 & < 2.0 &    &     5718 &     4.62 &      KIC \\
 KOI-5850 &  10991389 & 5611 & 4.35 & -0.01 & < 2.0 &    &     5945 &     4.46 &      P12 \\
 KOI-5855 &  11036168 & 5661 & 4.39 &  0.04 & < 2.0 &    &     5581 &     4.88 &      KIC \\
 KOI-5877 &  11183752 & 5539 & 4.51 & -0.00 & < 2.0 &    &     5568 &     4.46 &      KIC \\
 KOI-5888 &  11348610 & 5163 & 4.39 & -0.20 & < 2.0 &    &     5431 &     4.60 &      P12 \\
 KOI-5900 &  11453930 & 6277 & 4.24 & -0.18 &  12.7 &    &     6825 &     4.23 &      P12 \\
 KOI-6102 &   3545840 & 6518 & 4.03 &  0.03 &  11.4 &    &     6706 &     4.15 &      P12
