# Supplementary material for: Prevalence of Earth-size Planets Orbiting Sun-like Stars
Source: arXiv:1510.03902 source file (2015-10-13)
Supplement: Supplementary file 3 [file table_vonBraun.tex]

48737 &     6478 &    5728 &     3.92 &         &   0.14 & -0.38 &  66.4 \\
  10476 &     5242 &    5251 &     4.56 &    4.51 &  -0.02 &  0.01 &   0.0 \\
 216956 &     8459 &         &          &         &   0.20 & -0.92 &  73.0 \\
  GL144 &     5077 &    5137 &     4.61 &    4.63 &  -0.06 & -0.00 &   0.0 \\
  22484 &     5998 &    5966 &     4.14 &    4.08 &  -0.09 & -0.05 &   3.2 \\
  34411 &     5774 &    5794 &     4.27 &    4.13 &   0.05 &  0.06 &   0.0 \\
 143761 &     5627 &    5746 &     4.26 &    4.16 &  -0.22 & -0.23 &   0.0 \\
  38858 &     5646 &    5614 &     4.48 &    4.18 &  -0.22 & -0.28 &   0.0 \\
  GL699 &     3222 &         &     5.27 &         &  -0.39 &       &   4.7 \\
  16765 &     6356 &    6323 &     4.34 &    4.40 &  -0.15 & -0.03 &  32.3 \\
 186408 &     5760 &    5777 &     4.31 &    4.25 &   0.05 &  0.10 &   2.1 \\
  19373 &     5832 &    5992 &     4.23 &    4.19 &   0.08 &  0.13 &   3.2 \\
   1461 &     5386 &    5756 &     4.33 &    4.35 &   0.16 &  0.20 &   1.2 \\
 190406 &     5763 &    5979 &     4.39 &    4.44 &   0.03 &  0.06 &   2.0 \\
 210702 &     4780 &    5030 &     3.31 &    3.30 &   0.03 &  0.10 &   2.4 \\
  GL876 &     3129 &         &     5.19 &         &   0.19 &       &   5.6 \\
 157214 &     5738 &    5569 &     4.39 &    3.83 &  -0.37 & -0.39 &   0.0 \\
 115617 &     5538 &    5599 &     4.46 &    4.34 &   0.01 & -0.01 &   0.0 \\
  58946 &     6738 &    6430 &     4.13 &    4.09 &  -0.25 & -0.40 &  58.2 \\
  69897 &     6130 &    6185 &     4.23 &    4.25 &  -0.26 & -0.31 &   4.4 \\
  16895 &     6153 &    6258 &     4.29 &    4.26 &   0.00 & -0.00 &   8.4 \\
 107383 &     4705 &    4921 &     2.87 &    2.69 &  -0.30 & -0.18 &   3.3 \\
 177153 &     5909 &    6017 &     4.29 &    4.25 &  -0.06 & -0.06 &   3.0 \\
 173667 &     6296 &    6344 &     4.01 &    4.10 &  -0.03 & -0.03 &  17.3 \\
 168151 &     6221 &    6277 &     4.09 &    4.18 &  -0.28 & -0.39 &   7.9 \\
  23249 &     4955 &    5109 &     3.95 &    3.74 &   0.12 &  0.15 &   1.4 \\
   GL53 &     5348 &    5294 &     4.58 &    4.21 &  -0.68 & -0.76 &   0.0 \\
 161797 &     5502 &    5633 &     4.09 &    4.02 &   0.23 &  0.32 &   0.0 \\
  10700 &     5290 &    5244 &     4.57 &    4.17 &  -0.48 & -0.50 &   0.0 \\
   4614 &     5973 &    5835 &     4.42 &    4.35 &  -0.28 & -0.30 &   0.0 \\
  86728 &     5619 &    5766 &     4.31 &    4.29 &   0.19 &  0.21 &   1.2 \\
 126660 &     6211 &    6251 &     4.11 &    4.15 &  -0.02 &  0.02 &  29.7 \\
 186427 &     5678 &    5738 &     4.36 &    4.32 &   0.04 &  0.08 &   0.0 \\
 GL338B &     3867 &         &     4.75 &    3.89 &  -0.15 & -0.81 &   5.2 \\
  82328 &     6238 &    6155 &     3.94 &    3.95 &  -0.16 & -0.21 &   8.0 \\
 131156 &     5483 &    5572 &     4.53 &    4.67 &  -0.14 & -0.06 &   3.6 \\
 182736 &     5239 &    5291 &     3.81 &    3.67 &  -0.06 & -0.10 &   0.8 \\
 GL702A &     5407 &    5399 &     4.55 &    4.58 &   0.03 &  0.13 &   0.0 \\
  21019 &     5261 &    5422 &     3.85 &    3.65 &  -0.41 & -0.43 &   1.0 \\
 222368 &     6192 &    6136 &     4.15 &    4.11 &  -0.14 & -0.12 &   6.4 \\
  75732 &     5172 &    5330 &     4.49 &    4.34 &   0.35 &  0.39 &   0.0 \\
 130948 &     5787 &    6029 &     4.38 &    4.54 &  -0.05 &  0.02 &   6.1 \\
  39587 &     5898 &    6006 &     4.47 &    4.59 &  -0.04 &  0.01 &   8.8 \\
  GL687 &     3413 &         &     4.95 &         &  -0.09 &       &   5.5 \\
  30652 &     6441 &    6405 &     4.30 &    4.27 &   0.00 &  0.01 &  17.2 \\
 117176 &     5406 &    5496 &     4.01 &    3.82 &  -0.06 & -0.05 &   0.1 \\
 158633 &     5203 &    5197 &     4.58 &    4.29 &  -0.41 & -0.42 &   0.0 \\
    166 &     5327 &    5618 &     4.50 &    4.68 &   0.08 &  0.18 &   2.9 \\
 217107 &     5391 &    5652 &     4.34 &    4.26 &   0.31 &  0.35 &   0.0 \\
  10697 &     5442 &    5690 &     4.02 &    4.04 &   0.12 &  0.17 &   1.8 \\
   6210 &     6089 &    5970 &     3.84 &    3.74 &  -0.01 &  0.05 &  45.0 \\
 173701 &     5297 &    5448 &     4.48 &    4.42 &   0.24 &  0.37 &   0.0
